# Supplementary material for: Simulation Method of Microscale Fluid-Structure Interactions: Diffuse-Resistance-Domain Approach
Source: arXiv:2407.14291 source file (2025-08-07)
Supplement: Supplementary file 1 [file DRD_SM.pdf]

# Supplemental Information for “Simulation Method of Microscale Fluid-Structure Interactions: Diffuse-Resistance-Domain Approach”

Min Gao,<sup>1</sup> Zhihao Li,<sup>2,3</sup> and Xinpeng Xu<sup>3,4,\*</sup>

<sup>1</sup>*School of General Studies, Guangzhou College of Technology and Business,  
5 Guangming Road, Guangzhou, Guangdong 510850, China*

<sup>2</sup>*Department of Civil Engineering, Shantou University,  
243 Daxue Road, Shantou, 515063, Guangdong, China*

<sup>3</sup>*Department of Physics, Guangdong Technion - Israel Institute of Technology,  
241 Daxue Road, Shantou, Guangdong 515063, China*

<sup>4</sup>*Technion – Israel Institute of Technology, Haifa 3200003, Israel*  
(Dated: July 18, 2024)

## CONTENTS

|                                                                                      |    |
|--------------------------------------------------------------------------------------|----|
| I. Diffuse-resistance-domain (DRD) approach in a nutshell                            | 2  |
| A. Non-equilibrium thermodynamic framework based Onsager’s theory                    | 2  |
| B. Solving 1D diffusion equation                                                     | 3  |
| C. Solving Navier-Stokes equation: Fluid Particle Dynamics                           | 5  |
| II. DRD approach of simulating mFSI                                                  | 6  |
| A. Distinctive features of the DRD approach                                          | 6  |
| B. Governing equations derived from Onsager’s variational principle                  | 7  |
| C. Solid domains with prescribed translational and rotational velocities             | 10 |
| D. Capillary force on the spherical particle at the fluid-fluid interface            | 10 |
| III. Benchmark simulation 1: COMPLICATED (moving) solid geometries                   | 11 |
| A. Governing dynamic equations                                                       | 11 |
| B. Particle focusing in 2D microchannels                                             | 12 |
| IV. Benchmark simulation 2: Deformable (active) objects                              | 13 |
| A. Governing dynamic equations                                                       | 13 |
| B. Particle-based models for deformable (active) objects                             | 14 |
| C. Far-field dipolar flow field surrounding dumbbell microswimmers                   | 16 |
| V. Benchmark simulation 3: Two-phase flows on solid surfaces                         | 17 |
| A. Governing dynamic equations                                                       | 17 |
| B. Sharp-interface limit and generalized Navier boundary conditions (GNBC)           | 18 |
| C. Equilibrating dynamics of sessile droplets on planar surfaces                     | 19 |
| VI. Benchmark simulation 4: Reactive porous-media flows with evolving solid surfaces | 19 |
| A. Governing dynamic equations                                                       | 19 |
| B. Precipitation dynamics in 1D                                                      | 21 |
| Supplementary References                                                             | 23 |

In this Supplementary Information, we provide more details of the diffuse-resistance-domain (DRD) approach, discuss its applications in various fields, and validate the approach with some benchmark simulations. In Sec. I, we explain the idea of the DRD approach in a nutshell by solving the one-dimensional (1D) diffusion equation with three typical types of boundary conditions. In Sec. II, we apply the DRD approach to the direct numerical simulations (DNS) of microscale fluid-structure interactions (mFSI) where multiphase flows are involved, and the fluid-fluid interfacial

---

\* Corresponding authors; [xu.xinpeng@gtiit.edu.cn](mailto:xu.xinpeng@gtiit.edu.cn)

dynamics is closely coupled with wetting dynamics on solid surfaces, the contact line motion, and the dynamics of suspending objects. We first explain the distinctive features of the DRD approach and use Onsager's variational principle to derive the general governing equations. Then, in Secs. III-V, we numerically solve the governing equations derived in Sec. II and carry out some benchmark simulations of some specific mFSI problems taken from different research fields: (1) Particle focusing in microchannels from microfluidics. (2) Far-field dipolar flow field generated by a dumbbell microswimmer from active matter physics and microbiology. (3) Equilibrating dynamics of sessile droplets on planar solid surfaces from various contexts, *e.g.*, microscale manufacturing, petroleum production, and geophysics, *etc.* Finally, in Sec. VI, we show that our DRD approach can also be applied to study more complex mFSI where the solid structure evolves in time due to reactions or phase transitions such as crystal growth & melting, and precipitation & dissolution in porous-media, *etc.*

## I. DIFFUSE-RESISTANCE-DOMAIN (DRD) APPROACH IN A NUTSHELL

### A. Non-equilibrium thermodynamic framework based Onsager's theory

We study the non-equilibrium dynamics of mFSI in the framework of Onsager's linear response theory. To be comprehensive, we first outline the major components of Onsager's theory [S1–S3].

Consider a general non-equilibrium system that is characterized by a set of coarse-grained, slow-state variables,  $\alpha \equiv \{\alpha_1, \alpha_2, \dots\}$ . For small deviations near equilibrium, the system is in the linear response regime and the state  $\alpha$  evolves according to the linear kinetic equations [S1]:

$$X_i = \mathcal{R}_{ij} \dot{\alpha}_j, \quad (\text{S1})$$

where  $X_i$  are thermodynamic forces conjugate to thermodynamic fluxes or rates  $\dot{\alpha}_i$ , and, according to Onsager [S1], the resistance coefficients  $\mathcal{R}_{ij}$  form a symmetric and positive definite matrix. Off-diagonal entries  $\mathcal{R}_{ij}$  are referred to as cross-coupling coefficients between different irreversible processes labeled by  $i$  and  $j$  (with  $i \neq j$ ). Typical linear kinetic laws of Onsager's form include Fick's law of diffusion, Fourier's law of heat conduction, Newton's law of viscosity, and Ohm's law of electrical conduction, *etc.*

In this work, we propose a generic framework for the direct simulation of fluid-(solid)structure interactions at microscales that we call *diffuse-resistance-domain (DRD) approach*. It has two key features as follows. Firstly, we follow the idea of the phase-field approach where the fluid-solid interface is treated as a smooth *diffuse* interface (of small but non-zero thickness) and characterized by a phase parameter  $\psi$ . Secondly, the governing dynamic equations apply to both fluid and solid domains but have a large contrast in their *resistance* coefficients. The resistance coefficients are taken as functions of  $\psi$  that interpolate smoothly over different domains: the fluid domain, the fluid-solid interfacial domain (if needed to include), and the solid domain. In this section, we explain the DRD approach in a nutshell by using it to solve the one-dimensional (1D) diffusion equation with three typical types of boundary conditions.

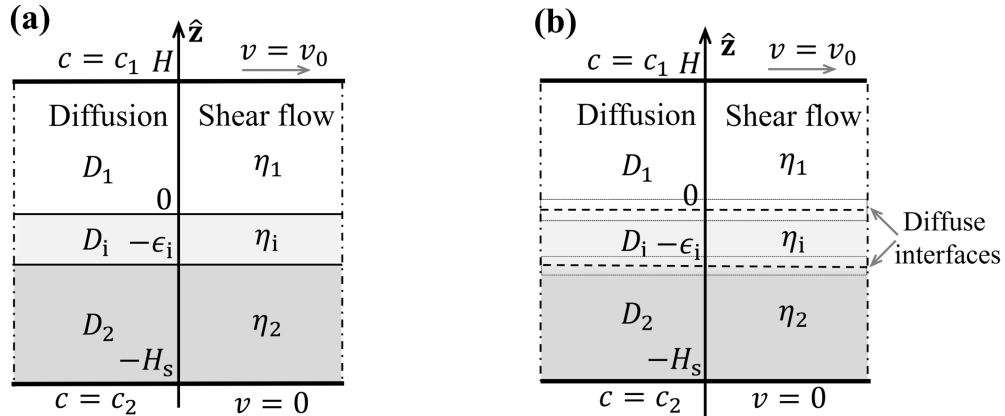

FIG. S1. Schematic illustrations of the 1D boundary value problem in a system including three (fluid, intermediate, and solid) domains with (a) sharp interfaces and (b) diffuse interfaces, respectively. The discussions and conclusions about the diffusion equation for 1D diffusion apply equally to the Stokes equation for laminar simple shear flow.

## B. Solving 1D diffusion equation

Consider one-dimensional (1D) diffusion in a fluid domain with  $0 \leq z \leq H$ , as shown in Fig. S1. The governing equation for concentration  $c = c(z, t)$  is the following 1D diffusion equation

$$\partial_t c = \partial_z (D \partial_z c), \quad (\text{S2})$$

subject to the boundary condition  $c(H, t) = c_1$  and a proper boundary condition at the fluid-solid interface  $z = 0$ . Three typical types of boundary conditions are usually taken. (1) Dirichlet boundary condition:  $c(0, t) = c_2$ . (2) Neumann boundary condition:  $\partial_z c(0, t) = 0$ . (3) Robin boundary condition:  $\partial_z c(0, t) = c(0, t) - c_2$ . The numerical solution of such a 1D problem is simple and various algorithms have been developed. However, in a real three-dimensional (3D) system with complicated curved solid geometries, the numerical solution becomes more challenging. To make the numerical solution easier, we propose the DRD approach to solve the 1D diffusion equation.

According to the DRD approach, firstly, we treat the fluid-solid interface at  $z = 0$  as a diffuse interface of small finite thickness  $\epsilon_s$ , characterized by a smooth interfacial profile function  $\psi$  (also called phase parameter as in the phase-field approach of multiphase flows [S4]) taking the form of

$$\psi(z) = \frac{1}{2} \left[ 1 - \tanh \left( \frac{z}{\sqrt{2}\epsilon_s} \right) \right], \quad (\text{S3})$$

that changes smoothly from  $\psi = 0$  in the fluid domain to  $\psi = 1$  in the solid domain. Secondly, to reproduce the three types of boundary conditions mentioned above at  $z = 0$ , we need to take proper smooth interpolations of the diffusivity  $D$  over different domains. For the Dirichlet and the Neumann boundary conditions, we choose a smooth interpolation of  $D(z)$  by taking it as a simple linear function of  $\psi$ :

$$D(\psi) = D_1 + (D_2 - D_1) \psi, \quad (\text{S4})$$

with  $D(\psi = 0) = D_1$  and  $D(\psi = 1) = D_2$  in the fluid and solid domains, respectively. In this case, if  $D_2 \gg D_1$  (and for small enough interfacial thickness  $\epsilon_s$ ) we reproduce the Dirichlet boundary condition at  $z = 0$  effectively as shown in Fig. S2(a) and Fig. S2(b). Whereas, if  $D_2 \ll D_1$  (and for small enough interfacial thickness  $\epsilon_s$ ), we would reproduce the Neumann boundary condition at  $z = 0$  effectively as shown in Fig. S2(c) and Fig. S2(d). In contrast, to reproduce the Robin boundary condition, we have to take an interpolation of  $D$  over three subdomains: the fluid domain, the fluid-solid interfacial domain, and the solid domain, in which the diffusivity  $D_i$  in the interfacial domain is very small:  $D_i < D_1 \ll D_2$ . In our simulations, we take the following interpolation form as shown in Fig. S3(a)

$$D(\psi) = \begin{cases} D_1 + 2\psi(D_i - D_1) & \text{if } \psi \leq 0.5 \text{ and } \psi = \psi_1, \\ 2D_i - D_2 + 2\psi(D_2 - D_i) & \text{if } \psi > 0.5 \text{ and } \psi = \psi_2, \end{cases} \quad (\text{S5})$$

with  $\psi_1(z) = \frac{1}{4} [1 - \tanh((z - \epsilon_i/2)/\sqrt{2}\epsilon_s)]$  and  $\psi_2(z) = \frac{1}{4} [3 - \tanh((z + \epsilon_i/2)/\sqrt{2}\epsilon_s)]$  both taking the similar form of Eq. (S3).

As shown in Figs. S2 and Figs. S3, we see that if we choose proper values of  $D_2/D_1$  and  $D_i/D_1$ , the steady-state numerical solutions (for  $0 \leq z \leq H$ ) obtained from the DRD approach can agree very well with the analytical steady-state solutions for the 1D diffusion equation under the three different types of boundary conditions. The validity of the DRD approach can be understood by considering the solutions of the 1D diffusion equation (S2) in a triple-domain system (for  $-H_s \leq z \leq H$ ) as shown in Fig. S1, where the two ‘‘sharp’’ interfaces are located at  $z = 0$  and  $z = -\epsilon_i$ , and  $D(z)$  is the diffusivity that varies piecewisely from  $D_1$  in the fluid domain ( $0 \leq z \leq H$ ), to  $D_i$  in the fluid-solid interfacial domain ( $-\epsilon_i \leq z < 0$ ), and to  $D_2$  in the solid domain ( $-H_s \leq z < -\epsilon_i$ ). Under the boundary conditions  $c(H, t) = c_1$  and  $c(-H_s, t) = c_2$ , we obtain the steady-state solution of the 1D diffusion equation (S2) as

$$c(z, t \rightarrow \infty) = \begin{cases} c_1 - (J_0/D_1)(H - z) & \text{if } 0 \leq z \leq H, \\ c_1 - (J_0/D_1)(H - D_1 z/D_i) & \text{if } -\epsilon_i \leq z < 0, \\ c_2 + (J_0/D_2)(z + H_s) & \text{if } -H_s \leq z < -\epsilon_i, \end{cases} \quad (\text{S6})$$

with the steady state flux  $J_0$  given by  $J_0 = D_1(c_1 - c_2)/[D_1\epsilon_i/D_i + H + (D_1/D_2)(H_s - \epsilon_i)]$ . We consider several special cases and pay attention to the effects of the relative magnitudes of the diffusivity  $r_D \equiv D_2/D_1$  in the solid domain (domain-2) and  $r_{D_i} \equiv D_i/D_1$  in the interfacial domain on the solution in the fluid domain (domain-1) as follows.

- Double-domain case 1 ( $\epsilon_i = 0$ ): the solid domain-2 has a very large diffusivity, *i.e.*,  $r_D = D_2/D_1 \gg 1$ . In this case, we find the solution (S6) in the fluid domain ( $0 \leq z \leq H$ ) reduces to be  $c \approx c_1 - (c_1 - c_2)(H - z)/H$ . That is,  $r_D = D_2/D_1 \gg 1$  sets an effective Dirichlet boundary condition at the interface  $z = 0$  for the diffusion in the fluid domain-1 (with  $0 \leq z \leq H$ ):

$$c(z = 0) = c_2, \quad (\text{S7a})$$

Alternatively, we can understand the result in another way. In the steady state, the diffusion flux is a constant:  $J = D(z)\partial_z c = J_0 = \text{const.}$ . Particularly in solid domain-2 with  $D(z) = D_2 \gg D_1$ , we have  $\partial_z c \rightarrow 0$  and hence  $c(z \leq 0) \approx c_2$  in the solid domain, yielding the effective Dirichlet boundary condition  $c(z = 0) = c_2$ .

Such an analytical result in the limit of  $r_D = D_2/D_1 \gg 1$  explains the numerical solution of the 1D diffusion equation using the DRD approach as shown in Figs. S2(a,b), where the numerical steady-state solution agrees very well with the analytical steady-state solution in the fluid domain ( $0 \leq z \leq H$ ) with Dirichlet boundary condition  $c(z = 0) = c_2$ .

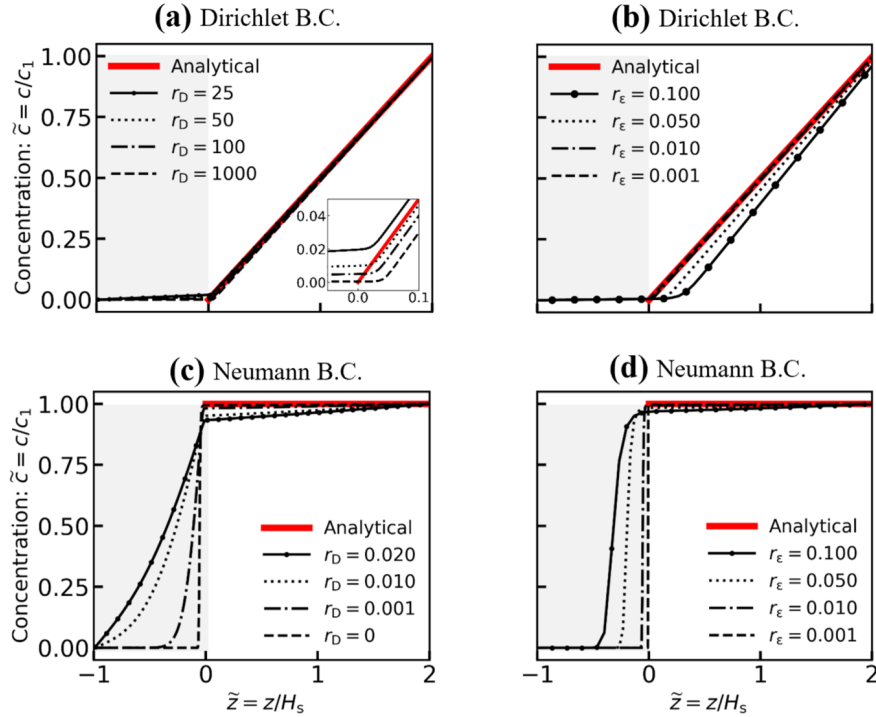

FIG. S2. Steady-state solutions  $\tilde{c}(z)$  of the 1D diffusion equation (S2) in the fluid domain  $0 \leq z \leq H$  under (a,b) Dirichlet and (c,d) Neumann boundary conditions. Numerical solutions using the DRD approach for different diffusivity ratios  $r_D = D_2/D_1$  and relative interface thicknesses  $r_\epsilon = \epsilon_s/H_s$  are compared to the analytical solution (red solid curves). For small enough  $r_{\epsilon s} \leq 0.01$ , (a,b) if  $r_D \gg 1$ , we reproduce Dirichlet boundary condition, while (c,d) if  $r_D \rightarrow 0$ , we reproduce Neumann boundary condition. Here, in (a,c), we fix  $r_\epsilon = 0.01$ , in (b) we fix  $r_D = 100$ , and in (d) we fix  $r_D = 0$  respectively.

- Double-domain case 2 ( $\epsilon_i = 0$ ): the solid domain-2 has a very small diffusivity, *i.e.*,  $r_D = D_2/D_1 \ll 1$ . In this case, the solution (S6) in the fluid domain-1 ( $0 \leq z \leq H$ ) reduces to be  $c \approx c_1$ . That is,  $r_D = D_2/D_1 \rightarrow 0$  sets an effective Neumann (impermeable zero-flux) boundary condition at the interface  $z = 0$  for the diffusion in the fluid domain-1 (with  $0 \leq z \leq H$ ):

$$D_1 \partial_z c|_{z=0} = 0, \quad (\text{S7b})$$

Alternatively, we can understand the result in another way. In the steady state and in the solid domain-2 with  $D(z) = D_2 \rightarrow 0$ , we have  $J = D_2 \partial_z c \rightarrow 0$ , yielding the effective Neumann boundary condition  $D_1 \partial_z c|_{z=0} = 0$ .

Such an analytical result in the limit of  $r_D = D_2/D_1 \rightarrow 0$  explains the numerical solution of the 1D diffusion equation using the DRD approach as shown in Figs. S2(c,d), where the numerical steady-state solution agrees very well with the analytical steady-state solution in the fluid domain ( $0 \leq z \leq H$ ) with the Neumann boundary condition  $\partial_z c|_{z=0} = 0$ .

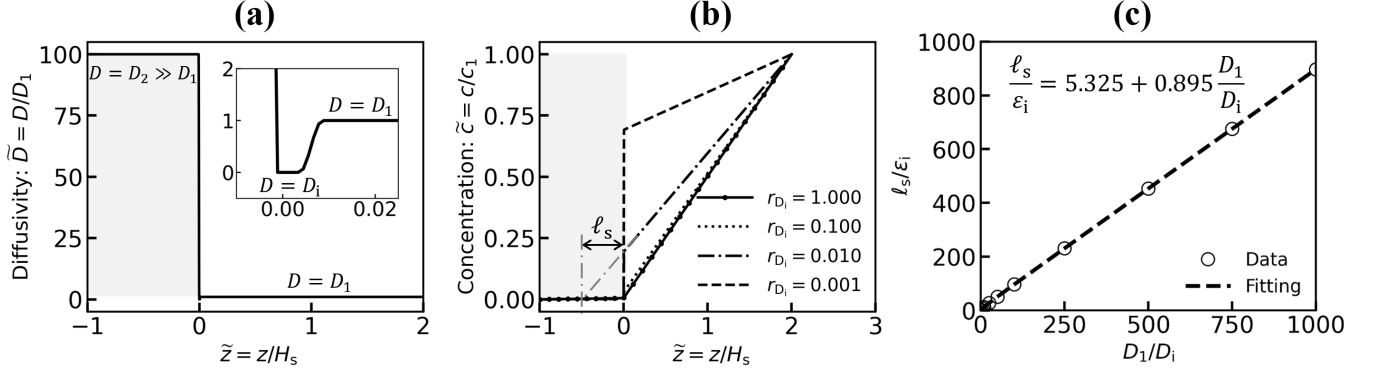

FIG. S3. Steady-state solutions  $\tilde{c}(z)$  of the 1D diffusion equation (S2) in the fluid domain  $0 \leq z \leq H$  under the Robin boundary condition. Numerical solutions are obtained using the DRD approach for different diffusivity ratios  $r_{D_i} = D_i/D_1$ . (a) The interpolation profile of the diffusivity  $D(z)$  used in the DRD numerical solution where we fix  $r_D = D_2/D_1 = 100$ ,  $r_e = 0.01$ , and vary  $r_{D_i}$ . (b) For different  $r_{D_i}$ , we reproduce the “slip” solution for Robin boundary condition. (c) The relative “slip” length  $\ell_s/\epsilon_i$  is found to be linearly proportional to  $D_1/D_i = r_{D_i}^{-1}$ , as predicted by sharp-interface calculations in the triple-domain system.

- Triple-domain case ( $\epsilon_i \ll H$  but  $\epsilon_i \neq 0$ ): the solid domain-2 has a very large diffusivity but the fluid-solid interfacial domain has a small diffusivity, *i.e.*,  $D_1 < D_1 \ll D_2$  or  $r_D = D_2/D_1 \gg 1$  and  $r_{D_i} = D_i/D_1 < 1$ . In this case, the solution (S6) in the fluid domain-1 ( $0 \leq z \leq H$ ) reduces to be  $c \approx c_1 - (c_1 - c_2)(H - z)/(H + \ell_s)$  with  $\ell_s \equiv D_1\epsilon_i/D_i$  and hence  $\ell_s/\epsilon_i = D_1/D_i > 1$ . That is,  $r_D = D_2/D_1 \gg 1$  and  $r_{D_i} = D_i/D_1 < 1$  together set an effective Robin (concentration “slip”) boundary condition at the interface  $z = 0$  for the diffusion in the fluid domain-1 (with  $0 \leq z \leq H$ ):

$$\ell_s \partial_z c|_{z=0} = c(z=0) - c_2, \quad (\text{S7c})$$

A similar alternative way of understanding the effective Robin boundary condition can be made as follows. Firstly, as discussed in the above double-domain case 1,  $r_D = D_2/D_1 \gg 1$  sets  $c(z \leq -\epsilon_i) = c_2$ . Secondly, in the steady state, the diffusion flux is a constant:  $J = D(z)\partial_z c = J_0$  and hence at the interface  $z = 0$ , we have  $D_1 \partial_z c|_{z=0+} = D_i \partial_z c|_{z=0-} = D_i [c(z=0^+) - c_2]/\epsilon_i$ , which gives the effective Robin boundary condition at  $z = 0$ :  $\ell_s \partial_z c|_{z=0+} = c(z=0^+) - c_2$ .

Again, such an analytical result explains the numerical solution of the 1D diffusion equation using the DRD approach as shown in Figs. S3(b), where the numerical steady-state solution agrees very well with the analytical steady-state solution in the fluid domain ( $0 \leq z \leq H$ ) with the Robin boundary condition  $\ell_s \partial_z c|_{z=0} = c(z=0) - c_2$ . Moreover, the linear dependence of the slip length  $\ell_s/\epsilon_i = D_1/D_i > 1$  on  $r_{D_i}^{-1} = D_1/D_i$  has also been confirmed numerically as shown in Figs. S3(c).

### C. Solving Navier-Stokes equation: Fluid Particle Dynamics

The idea of the DRD approach mentioned above can also be used to numerically solve the dynamic equations for other transport phenomena such as the heat conduction equation, Navier-Stokes equation, electrokinetic equation, and so on. Here, we present another example of the application of the DRD approach to solve the Navier-Stokes equations.

To be specific, we consider the 1D laminar flow field (with velocity  $\mathbf{v} = v(z, t)\hat{\mathbf{x}}$  and pressure  $p = \text{const}$ ), which is induced by simple shear in a viscous fluid (with  $0 \leq z \leq H$ ) as shown in Fig. S1. The governing equation for the 1D velocity field is the following 1D Navier-Stokes equation

$$\partial_t v = \partial_z (\nu \partial_z v), \quad (\text{S8})$$

which takes the same form of the 1D diffusion equation (S2) with  $\nu$  being the kinematic viscosity. When Eq. (S8) is subject to the boundary condition  $v(H, t) = V_0$  and one of the three types of boundary conditions for  $v$  at the fluid-solid interface  $z = 0$ , we can then use the DRD approach to solve it numerically as discussed above. All the above discussions for the solution of the 1D diffusion equation also apply to the solution of 1D Navier-Stokes equation here. The three types of boundary conditions at  $z = 0$  can be reproduced effectively if we take proper smooth interpolations of the viscosity  $\nu$  over different domains. For the interpolation form in Eq. (S4), if  $\nu_2 \gg \nu_1$  (and for small enough interfacial thickness  $\epsilon_s$ ), we reproduce the Dirichlet or no-slip boundary condition at  $z = 0$  effectively:  $v|_{z=0} = -V_0$ . Whereas, if  $\nu_2 \ll \nu_1$  (and for small enough interfacial thickness  $\epsilon_s$ ), we would reproduce the Neumann or free-surface boundary condition at  $z = 0$  effectively:  $\partial_z v|_{z=0} = 0$ . In contrast, for the interpolation form in Eq. (S5), if  $D_i < D_1 \ll D_2$ , we reproduce the Robin boundary condition – Navier’s slip boundary condition:  $\ell_s \partial_z v|_{z=0} = v(z=0) + V_0$ .

Finally, we would like to point out that similar ideas of using smoothed profiles of viscosity across the interfacial region have been proposed before to facilitate the numerical study of colloidal dynamics [S5, S6] (so-called fluid particle dynamics method, or FPD method), particle dispersion in nematic crystal liquid-solvent [S7], the impact of solid objects on free surfaces [S8, S9], two-phase flows in or on stationary solid domains with complicated geometries [S10], the melting and flowing of solids [S11], and the fluid-structure interaction in presence of a hyperelastic body [S12], *etc.* Particularly, the FPD method has been shown by careful numerical [S6, S13, S14] and analytical studies [S15] to be the capability of reproducing arbitrary flow fields derived from conventional sharp-interface methods as the viscosity ratio tends to be large enough and the interface thickness tends to be small enough.

## II. DRD APPROACH OF SIMULATING MFSI

### A. Distinctive features of the DRD approach

We now explain how to use the DRD approach to simulate mFSI as schematically shown in Fig. S4, where multiphase flows are involved, and the fluid-fluid interfacial dynamics is closely coupled with wetting dynamics on solid surfaces, the contact line motion, and the dynamics of suspending objects (*e.g.*, colloids, microswimmers, and flexible fibers).

Firstly, in the DRD approach, the fluid-fluid interfaces and the fluid-solid interfaces are both treated as diffuse interfaces with small finite thicknesses and characterized by smooth interfacial profile functions – phase parameters. Such a diffuse interface method with multiple phase parameters is usually referred to as multi-phase-field (MPF) method [S9, S10] and it has been widely used to simulate multiphase flows because of their advantages in avoiding explicit tracking of moving interfaces. For example, in the framework of the MPF method, the fluid-fluid-solid triple-phase system shown in Fig. S4 is regarded as ONE viscoelastic structured fluid with spatially varying viscosity and mobility, and the dynamic equations take the same form everywhere in the whole system. In contrast, in the DRD approach, although the dynamics of the fluid-fluid interface and the phase-field function  $\phi$  are described by the traditional diffuse-interface (Cahn-Hilliard) approach [S4, S16], yet the fluid-solid interfacial profile (phase-field parameter) function  $\psi$  is prescribed (not solved from dynamic equations such as Cahn-Hilliard equations [S9]) by

$$\psi(\mathbf{r}, t) = \frac{1}{2} \left[ 1 + \tanh \left( \frac{\mathcal{D}(\mathbf{r}, t)}{\sqrt{2}\epsilon_s} \right) \right], \quad (\text{S9})$$

that changes smoothly from  $\psi = 0$  in the fluid domain to  $\psi = 1$  in the solid domain. Here  $\epsilon_s$  characterizes the small interface thickness and  $\mathcal{D}(\mathbf{r}, t)$  is the signed distance function (at position  $\mathbf{r}$ ) away from the solid surface with  $\mathcal{D} > 0$  ( $< 0$ ) in the solid (fluid) domain. Note that, in general,  $\mathcal{D}(\mathbf{r}, t)$  is a function of time, representing moving or deforming solid surfaces, for example, rigid particles or flexible fibers moving in viscous fluids [S5, S6, S14], swimming microswimmers [S17], *etc.*

The idea of using a prescribed interfacial profile function to deal with fluid-solid interactions has been used in several different forms and contexts: the fluid-particle dynamics (FPD) method for the simulations of colloidal suspensions with hydrodynamic interactions in single-phase fluids [S5, S6], the modified ternary phase-field method [S10] and the diffuse domain method [S18, S19] for two-phase flows in or on stationary solid domains with complicated geometries. In contrast, in the DRD approach that extends the FPD method [S5, S6] to triple-phase flows, the solid domain can move or deform, while the description of moving & deforming solid domains is very difficult in the modified ternary phase-field method [S10]. Moreover, the dynamic equations take the same form everywhere in the whole system; by introducing spatially-varying viscosity and mobility, one doesn’t need to modify the equations using the fluid-solid interfacial profile function  $\psi$  as one has to do in the diffuse domain method [S18, S19].

Secondly, the spatially-varying viscosity and mobility are assumed to change smoothly from the viscosity  $\eta_f$  and mobility  $M_f$  in the two-fluids domain to the large viscosity  $\eta_s$  ( $\gg \eta_f$ ) and small mobility  $M_s$  ( $\ll M_f$ ) inside the



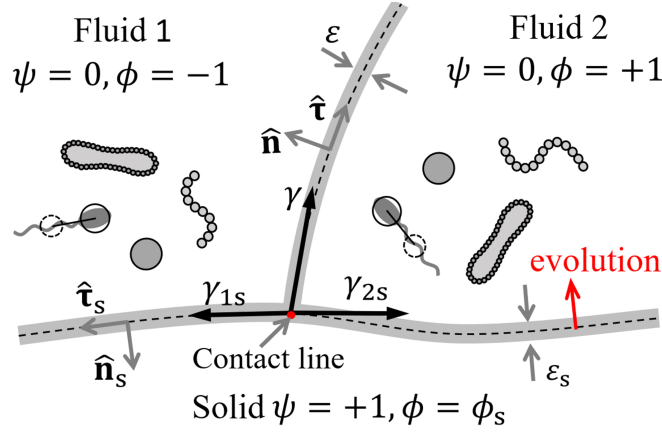

FIG. S4. Schematic illustration for typical scenarios of DRD approach in simulating mFSI where multiphase flows are involved, and the fluid-fluid interfacial dynamics is closely coupled with wetting dynamics and contact line motion on solid surfaces with complicated corrugated geometries, the dynamics of suspending (active deformable) objects (*e.g.*, rigid particles, microswimmers, flexible fibers, elastic capsules) as well as the evolving dynamics of solid surfaces due to precipitation & dissolution. The immiscible two-phase fluid regions are distinguished by different values of phase parameter  $\phi$ , while sharing the same value  $\psi = 0$ . The solid domain is represented by  $\psi = 1$  and  $\phi = \phi_s$ . Interfacial conditions are imposed effectively by smooth interpolations of dynamic-resistance coefficients over different domains.

rigid solid domain. The natural idea of using large viscosity to mimic & approximate the rigidity of solid domains upon shear forces has been employed in the simulations of several different systems such as colloidal suspensions with hydrodynamic interactions in single-phase fluids [S5, S6], the impact of solid objects on free surfaces [S8, S9], and two-phase flows in or on stationary solid domains with complicated geometries [S10]. In the DRD approach, the smooth profiles of viscosity  $\eta(\mathbf{r})$  and mobility  $M(\mathbf{r})$  are both chosen as a function of interfacial profile functions  $\phi$  and  $\psi$ :

$$\eta(\phi, \psi) = \eta_f(\phi) + [\eta_s - \eta_f(\phi)] \psi, \quad (\text{S10a})$$

$$M(\phi, \psi) = M_f(\phi) + [M_s - M_f(\phi)] \psi, \quad (\text{S10b})$$

with  $\eta(\phi, 0) = \eta_f(\phi)$ ,  $M(\phi, 0) = M_f(\phi)$ ,  $\eta(\phi, 1) = \eta_s$ , and  $M(\phi, 1) = M_s$  in the fluid and solid domains, respectively. Note that, as discussed in Sec. I, for the linear monotonic interpolation of  $\eta(\mathbf{r})$ , if  $\eta_s \gg \eta_f(\phi)$  and  $M_s \ll M_f(\phi)$ , we would reproduce the Dirichlet (no-slip and impermeability) boundary condition for the flow velocity  $\mathbf{v}$  and the Neumann (impermeability) boundary conditions for the phase field  $\phi$  at the surfaces of rigid solids [S5, S6, S20], respectively. However, if the fluid slip is important at the solid surfaces, we have to use a non-monotonic interpolation of  $\eta(\psi)$ , in which an intermediate thin layer of lubricant with a very small viscosity ( $\eta_i < \eta_f \ll \eta_s$ ) has to be included [S9, S13, S14], for example, we can use the interpolation form of Eq. (S5) [S13]

$$\eta(\phi, \psi) = \begin{cases} \eta_f(\phi) + 2\psi [\eta_i - \eta_f(\phi)] & \text{if } \psi \leq 0.5 \text{ and } \psi = \psi_1, \\ 2\eta_i - \eta_s + 2\psi (\eta_s - \eta_i) & \text{if } \psi > 0.5 \text{ and } \psi = \psi_2, \end{cases} \quad (\text{S11a})$$

with  $\psi_1(\mathbf{r}, t) = \frac{1}{4} \left[ 1 - \tanh \left( \frac{\mathcal{D}(\mathbf{r}, t) - \epsilon_i/2}{\sqrt{2}\epsilon_s} \right) \right]$  and  $\psi_2(\mathbf{r}, t) = \frac{1}{4} \left[ 3 - \tanh \left( \frac{\mathcal{D}(\mathbf{r}, t) + \epsilon_i/2}{\sqrt{2}\epsilon_s} \right) \right]$  both taking the similar form of Eq. (S9). Similarly, if the relaxation dissipation across the fluid-solid interface is critical, for example, during the contact line motion [S4], we choose the same interpolation form of mobility  $M(\psi)$  as Eq. (S11a):

$$M(\phi, \psi) = \begin{cases} M_f(\phi) + 2\psi [M_i - M_f(\phi)] & \text{if } \psi \leq 0.5 \text{ and } \psi = \psi_1, \\ 2M_i - M_s + 2\psi (M_s - M_i) & \text{if } \psi > 0.5 \text{ and } \psi = \psi_2, \end{cases} \quad (\text{S11b})$$

with  $M_s \ll M_f(\phi) < M_i$  as to be explained in Sec. VB.

## B. Governing equations derived from Onsager's variational principle

Now based on the ideas presented in the above subsection, we use Onsager's variational principle to derive the governing dynamic equations for the simulation of mFSI using the DRD approach [S2–S4, S21]. To be specific,

we consider an immiscible two-phase flow including  $N$  moving rigid spherical particles over a rigid corrugated solid boundary surface, as shown in Fig. S4. In the DRD approach, we use the interfacial profile functions or phase parameters  $\phi(\mathbf{r}, t)$ ,  $\psi_\alpha(\mathbf{r}, t)$  (with  $\alpha = 1, \dots, N$ ), and  $\psi(\mathbf{r})$  to describe the immiscible fluid-fluid interface, the surface of  $\alpha$ -th particle, and the corrugated solid boundary surface, respectively. The phase parameter  $\phi$  is locally conserved, following the conservation equation

$$\partial_t \phi + \mathbf{v} \cdot \nabla \phi = -\nabla \cdot \mathbf{J}, \quad (\text{S12})$$

with  $\mathbf{v}(\mathbf{r}, t)$  denoting the flow velocity field. For the  $\alpha$ -th particle of diameter  $d$  centered at  $\mathbf{R}_\alpha(t)$ , the interfacial profile function  $\psi_\alpha$  takes the form of Eq. (S9) with the signed distance function given by  $\mathcal{D}_\alpha(\mathbf{r}, t) = d/2 - |\mathbf{r} - \mathbf{R}_\alpha(t)|$ , that is,

$$\psi_\alpha(\mathbf{r}, t) = \frac{1}{2} \left[ 1 + \tanh \left( \frac{d/2 - |\mathbf{r} - \mathbf{R}_\alpha(t)|}{\sqrt{2}\epsilon_s} \right) \right], \quad (\text{S13})$$

and the velocity of the particle is given by

$$\dot{\mathbf{R}}_\alpha = \mathbf{V}_\alpha(t) \equiv \frac{\int d\mathbf{r}' \psi_\alpha \mathbf{v}(\mathbf{r}', t)}{\int d\mathbf{r}' \psi_\alpha}, \quad (\text{S14})$$

with the superscript dot denoting the time derivative afterward, *i.e.*,  $\dot{\mathbf{R}}_\alpha = d\mathbf{R}_\alpha/dt$ . For the corrugated solid boundary surface, the interfacial profile function  $\psi$  takes the form of Eq. (S9):  $\psi(\mathbf{r}, t) = \frac{1}{2} [1 + \tanh(\mathcal{D}(\mathbf{r}, t)/\sqrt{2}\epsilon_s)]$  with  $\mathcal{D}(\mathbf{r}, t)$  being the signed distance away from the nearest solid boundary surfaces.

The free energy for the fluid-fluid-solid triple-phase system includes three contributions:

$$\mathcal{F}[\phi(\mathbf{r}), \psi(\mathbf{r}), \psi_\alpha(\mathbf{r}; \mathbf{R}_\alpha)] = \mathcal{F}_b[\phi(\mathbf{r})] + \mathcal{F}_s[\phi(\mathbf{r}), \psi(\mathbf{r}), \psi_\alpha(\mathbf{r}; \mathbf{R}_\alpha)]. \quad (\text{S15})$$

Here  $\mathcal{F}_b[\phi(\mathbf{r})]$  is the Cahn-Hilliard free energy with the Landau-Ginzburg form of

$$\mathcal{F}_b[\phi(\mathbf{r})] = \int d\mathbf{r} \left[ f_b(\phi) + \frac{1}{2} K (1 - \psi) |\nabla \phi|^2 \right], \quad (\text{S16a})$$

where  $f_b(\phi) = \frac{1}{4} a (\phi^2 - 1)^2$  is the double-well potential and  $K$  is the (positive) interfacial stiffness parameter. The interfacial thickness and interfacial tension of fluid-fluid interface are given by  $\epsilon = \sqrt{K/a}$  and  $\gamma = 2\sqrt{2}a\epsilon/3 = 2\sqrt{2Ka}/3$ , respectively. The second term  $\mathcal{F}_s$  in the total free energy (S15) arises from the interfacial free energy at the fluid-solid interfaces

$$\mathcal{F}_s[\phi(\mathbf{r}), \psi(\mathbf{r}), \psi_\alpha(\mathbf{r}; \mathbf{R}_\alpha)] = \sum_{\alpha=1}^N \int d\mathbf{r} \epsilon_{s,\alpha} f_{s,\alpha}(\phi) |\nabla \psi_\alpha|^2 + \int d\mathbf{r} \epsilon_s f_s(\phi) |\nabla \psi|^2, \quad (\text{S16b})$$

where  $f_{s,\alpha}(\phi) = -\frac{1}{4}\gamma \cos \theta_{s,\alpha} (\phi^3 - 3\phi)$ , and  $f_s(\phi) = -\frac{1}{4}\gamma \cos \theta_s (\phi^3 - 3\phi)$  are the surface energy densities at the fluid-particle and fluid-solid interfaces, respectively, with  $\theta_{s,\alpha}$  and  $\theta_s$  being the static contact angles at the solid surfaces.

The rate of change of the total free energy  $\dot{\mathcal{F}}_T = \dot{\mathcal{F}} - \dot{\mathcal{W}}$  is then given by

$$\dot{\mathcal{F}}_T = \int d\mathbf{r} \hat{\mu}_T \partial_t \phi - \sum_{\alpha} \mathbf{F}_\alpha^{\text{tot}} \dot{\mathbf{R}}_\alpha, \quad (\text{S17})$$

where the total chemical potential,  $\hat{\mu}_T$ , is given by

$$\hat{\mu}_T \equiv \hat{\mu} + \sum_{\alpha=1}^N \epsilon_s \mu_{s,\alpha} |\nabla \psi_\alpha|^2 + \epsilon_s \mu_s |\nabla \psi|^2, \quad (\text{S18})$$

with  $\hat{\mu} = \mu - \nabla \cdot [K(1 - \psi)\nabla \phi]$ ,  $\mu = \partial f_b(\phi)/\partial \phi = a\phi(\phi^2 - 1)$ ,  $\mu_{s,\alpha} = \partial f_{s,\alpha}(\phi)/\partial \phi = -\frac{3}{4}\gamma \cos \theta_{s,\alpha}(\phi^2 - 1)$ , and  $\mu_s = \partial f_s(\phi)/\partial \phi = -\frac{3}{4}\gamma \cos \theta_s(\phi^2 - 1)$  being the generalized chemical potential for two-phase fluids, the chemical potential for homogeneous fluids, and the surface chemical potentials at the particle and solid boundary surfaces, respectively. Note that  $\hat{\mu}$  is related to the Korteweg capillary pressure tensor  $\mathbf{\Pi}$  [S6]

$$\mathbf{\Pi} \equiv \hat{p} + K \nabla \phi \nabla \phi, \quad (\text{S19})$$



by the generalized Gibbs-Duhem relation

$$\phi \nabla \hat{\mu} = \nabla \cdot \mathbf{\Pi}, \quad (\text{S20})$$

with the generalized pressure  $\hat{p} = -\hat{f} + \phi \hat{\mu} = p - \frac{1}{2}K |\nabla \phi|^2 - K \phi \nabla^2 \phi$  and  $p = -f + \phi \mu$ . The work power  $\dot{W} = \sum_{\alpha} \mathbf{F}_{\alpha}^{\text{tot}} \dot{\mathbf{R}}_{\alpha}$  is the work power done by “external forces”  $\mathbf{F}_{\alpha}^{\text{tot}}$  and the particle velocity  $\dot{\mathbf{R}}_{\alpha}$  is given in Eq. (S14) as a function of velocity field  $\mathbf{v}$ . The total force  $\mathbf{F}_{\alpha}^{\text{tot}}$  applied on the  $\alpha$ -th particle can be written generally as  $\mathbf{F}_{\alpha}^{\text{tot}} \equiv \mathbf{F}_{\alpha}^{\text{act}} - \partial U / \partial \mathbf{R}_{\alpha}$ , where  $\mathbf{F}_{\alpha}^{\text{act}}$  is the active or self-propelled forces (of biological or chemical origin) applied on the  $\alpha$ -th particle and the interaction potential  $U(\{\mathbf{R}_{\alpha}\})$  is

$$U(\{\mathbf{R}_{\alpha}\}) = \sum_{\zeta > \beta} U_{\text{pp}}(|\mathbf{R}_{\zeta} - \mathbf{R}_{\beta}|) + \sum_{\beta} U_{\text{ps}}(|\mathcal{D}(\mathbf{R}_{\beta})|), \quad (\text{S21a})$$

where  $U_{\text{pp}}$  and  $U_{\text{ps}}$  denote the two-body particle-particle interactions and the particle-solid boundary interactions, respectively, and  $|\mathcal{D}(\mathbf{R}_{\beta})|$  denoting the minimal distance of the  $\beta$ -th particle at  $\mathbf{r} = \mathbf{R}_{\beta}$  away from the solid boundary. In this work, the following harmonic potentials are employed to take into account the excluded volume interactions between particles and between particles and solid boundaries:

$$U_{\text{pp}}(|\mathbf{R}_{\zeta} - \mathbf{R}_{\beta}|) = \begin{cases} \frac{k_s}{2d^2} (R_{\beta\zeta} - d)^2, & R_{\beta\zeta} \leq d, \\ 0, & R_{\beta\zeta} > d, \end{cases} \quad (\text{S21b})$$

$$U_{\text{ps}}(|\mathcal{D}(\mathbf{R}_{\beta})|) = \begin{cases} \frac{k_s}{2d^2} (|\mathcal{D}(\mathbf{R}_{\beta})| - d/2)^2, & |\mathcal{D}(\mathbf{R}_{\beta})| \leq d/2, \\ 0, & |\mathcal{D}(\mathbf{R}_{\beta})| > d/2, \end{cases} \quad (\text{S21c})$$

with  $R_{\beta\zeta} \equiv |\mathbf{R}_{\beta\zeta}|$  and  $\mathbf{R}_{\beta\zeta} \equiv \mathbf{R}_{\zeta} - \mathbf{R}_{\beta}$ . From Eqs. (S21), we then obtain

$$\begin{aligned} \mathbf{F}_{\alpha}^{\text{tot}} &= \mathbf{F}_{\alpha}^{\text{act}} - \sum_{\beta \neq \alpha} \frac{\partial U_{\text{pp}}}{\partial R_{\beta\alpha}} \hat{\mathbf{R}}_{\beta\alpha} - \frac{\partial U_{\text{ps}}}{\partial |\mathcal{D}(\mathbf{R}_{\alpha})|} (-\hat{\mathbf{n}}_{\text{s},\alpha}), \\ &= \mathbf{F}_{\alpha}^{\text{act}} - \sum_{\beta \neq \alpha} \frac{k_s}{d^2} (R_{\beta\alpha} - d) \hat{\mathbf{R}}_{\beta\alpha} - \frac{k_s}{d^2} (|\mathcal{D}(\mathbf{R}_{\alpha})| - d/2) (-\hat{\mathbf{n}}_{\text{s},\alpha}), \end{aligned} \quad (\text{S22})$$

with  $\hat{\mathbf{R}}_{\beta\alpha} \equiv \mathbf{R}_{\beta\alpha} / R_{\beta\alpha}$ . Submitting Eqs. (S12) and (S14) into Eq. (S17), we obtain

$$\dot{\mathcal{F}}_{\text{T}}[\mathbf{v}, \mathbf{J}] = \int d\mathbf{r} \left[ (-\hat{\mu}_{\text{T}} \mathbf{v} \cdot \nabla \phi - \hat{\mu}_{\text{T}} \nabla \cdot \mathbf{J}) - \sum_{\alpha} \frac{\psi_{\alpha}(\mathbf{v} \cdot \mathbf{F}_{\alpha}^{\text{tot}})}{\int d\mathbf{r}' \psi_{\alpha}} \right], \quad (\text{S23})$$

and the dissipation function is given by

$$\Phi[\mathbf{v}, \mathbf{J}] = \int d\mathbf{r} \left[ \frac{1}{4} \eta (\nabla \mathbf{v} + \nabla \mathbf{v}^{\text{T}})^2 + \frac{\mathbf{J}^2}{2M} \right], \quad (\text{S24})$$

with the superscript T denoting the tensor transpose. Furthermore, imposing the incompressibility condition  $\nabla \cdot \mathbf{v} = 0$ , we obtain the Rayleighian

$$\mathcal{R}[\mathbf{v}, \mathbf{J}] = \dot{\mathcal{F}}_{\text{T}} + \Phi - \int d\mathbf{r} p \nabla \cdot \mathbf{v}, \quad (\text{S25})$$

with  $p$  being a local Lagrange multiplier and representing the pressure. Minimizing  $\mathcal{R}$  with respect to  $\mathbf{v}$  and  $\mathbf{J}$  gives

$$\rho (\partial_t \mathbf{v} + \mathbf{v} \cdot \nabla \mathbf{v}) = -\nabla p + \nabla \cdot [\eta (\nabla \mathbf{v} + \nabla \mathbf{v}^{\text{T}})] + \hat{\mu}_{\text{T}} \nabla \phi + \sum_{\alpha=1}^N \frac{\psi_{\alpha} \mathbf{F}_{\alpha}^{\text{tot}}}{\int d\mathbf{r}' \psi_{\alpha}}, \quad (\text{S26a})$$

$$\partial_t \phi + \mathbf{v} \cdot \nabla \phi = \nabla \cdot (M \nabla \hat{\mu}_{\text{T}}), \quad (\text{S26b})$$

where we have added the inertial terms in Eq. (S26a) and  $\rho$  is the mass density of the fluid.

In summary, the governing dynamic equations for the immiscible two-phase flows including  $N$  suspending particles over a stationary rigid corrugated solid surface include Eqs. (S26), (S18), (S22), and the incompressibility condition  $\nabla \cdot \mathbf{v} = 0$ , supplemented with proper initial and boundary conditions at the boundary of the whole computational domain.

### C. Solid domains with prescribed translational and rotational velocities

In our simulations, the velocities of solid domains are obtained by different methods for the following different cases. Firstly, the solid domain moves autonomously with surrounding fluids such as the motion of suspending colloidal particles or flexible fibers in viscous fluids. In this case, the particle velocity is computed directly from Eq. (S14).

Secondly, the solid domain is stationary or moving with prescribed velocities. In this case, if the boundary of the solid domain overlaps that of the computational domain, such stationary conditions can be imposed by applying boundary conditions of zero or some prescribed velocity. However, if the solid domain is inside the computational domain such as suspending particles or deformable objects, we have to employ different methods to impose the prescribed velocity, given by

$$\mathbf{v}_s(\mathbf{r}) = \mathbf{V}^* + \boldsymbol{\omega}^* \times (\mathbf{r} - \mathbf{R}_s). \quad (\text{S27})$$

with  $\mathbf{V}^*$  and  $\boldsymbol{\omega}^*$  being the translational and rotational velocities, respectively;  $\mathbf{R}_s$  being the rotation axis of the solid domain. Technically, to achieve the prescribed velocity  $\mathbf{v}_s(\mathbf{r})$  of solid domains, we use the following two different methods.

- *Method of velocity interpolation by two-step updates* [S13, S14]. We first use the velocity  $\mathbf{v}^n$  at time step  $n$  and solve the Navier-Stokes equation (S26a) to obtain an intermediate velocity  $\mathbf{v}_i^n$ . We then assume that the velocity  $\mathbf{v}^{n+1}$  at the next time step  $n+1$  is given by an interpolation [S22, S23] between the prescribed velocity  $\mathbf{v}_s$  and  $\mathbf{v}_i^n$  via

$$\mathbf{v}^{n+1}(\mathbf{r}) = \Theta[\psi(\mathbf{r})]\mathbf{v}_s(\mathbf{r}) + \{1 - \Theta[\psi(\mathbf{r})]\}\mathbf{v}_i^n(\mathbf{r}), \quad (\text{S28})$$

in which  $\Theta(\phi)$  is a Heaviside function with  $\Theta = 1$  for  $\psi \geq \psi_c$  and 0 for  $\psi < \psi_c$ . In our simulations, we take  $\psi_c = 0.95$  to be close to  $\psi = 1$ .

- *Method of introducing artificial, large friction term* [S24] in the Navier-Stokes equation (S26a):

$$\rho(\partial_t \mathbf{v} + \mathbf{v} \cdot \nabla \mathbf{v}) = -\nabla p + \nabla \cdot [\eta(\nabla \mathbf{v} + \nabla \mathbf{v}^T)] + \hat{\mu}_T \nabla \phi + \sum_{\alpha=1}^N \frac{\psi_\alpha \mathbf{F}_\alpha^{\text{tot}}}{\int d\mathbf{r}' \psi_\alpha} + \zeta_s \psi (\mathbf{v}_s - \mathbf{v}), \quad (\text{S29})$$

with  $\zeta_s$  being an artificial large friction coefficient.

### D. Capillary force on the spherical particle at the fluid-fluid interface

Consider a single spherical colloidal particle of diameter  $d$  that is located at  $\mathbf{R}_1$  and described by the phase parameter  $\psi_1(\mathbf{r}; \mathbf{R}_1)$ . We examine the equilibrium condition for the colloid particle when it is adsorbed to a planar fluid-fluid interface without external forces, *i.e.*,  $\mathbf{F}_1^{\text{tot}} = 0$ . In this case, the total free energy is given from Eq. (S15) by

$$\mathcal{F}[\phi(\mathbf{r}), \psi_1(\mathbf{r}; \mathbf{R}_\alpha)] = \int d\mathbf{r} \left[ f_b(\phi) + \frac{1}{2} K(1 - \psi) |\nabla \phi|^2 \right] + \int d\mathbf{r} \epsilon_s f_{s,1}(\phi) |\nabla \psi_1|^2, \quad (\text{S30})$$

where  $f_b(\phi) = \frac{1}{4} a (\phi^2 - 1)^2$  is the double-well potential and  $f_{s,1}(\phi) = -\frac{1}{4} \gamma \cos \theta_s (\phi^3 - 3\phi)$  is the surface energy densities at the fluid-particle interface with  $\theta_s$  being the static contact angle at the particle surface.

During an infinitesimal time interval  $\delta t$ , due to the presence of velocity field  $\mathbf{v}$ , the fluid-fluid phase field evolves as  $\delta \phi = -\delta t \mathbf{v} \cdot \nabla \phi$  and the particle displaces by  $\delta \mathbf{R}_1 = \delta t \int d\mathbf{r}' \psi_\alpha \mathbf{v}(\mathbf{r}', t) / \int d\mathbf{r}' \psi_\alpha$  as given in Eq. (S14). The change in the free energy  $\mathcal{F}$  in Eq. (S30) due to these changes is then given by

$$\delta \mathcal{F} = - \int d\mathbf{r} \delta t \mathbf{v} \cdot \left( \hat{\mu} \nabla \phi + \epsilon_s |\nabla \psi_1|^2 \nabla f_{s,1} \right), \quad (\text{S31})$$

or equivalently,

$$\delta \mathcal{F} = \int d\mathbf{r} \delta t \mathbf{v} \cdot \left( \nabla \cdot \boldsymbol{\Pi} - \frac{\partial \epsilon_s f_{s,1} |\nabla \psi_1|^2}{\partial \mathbf{R}_1} \right), \quad (\text{S32})$$

where we have used the generalized Gibbs-Duhem relation in Eq. (S20) and the identity  $\nabla |\nabla \psi_1|^2 = -\partial |\nabla \psi_1|^2 / \partial \mathbf{R}_1$ .

In the limits of sharp interface and large solid viscosity,  $\delta t \mathbf{v} \rightarrow \delta \mathbf{R}_1$  inside the particle using velocity continuity condition at the particle surface,  $\mathbf{v}_s = \dot{\mathbf{R}}_1$ , the change of the free energy becomes

$$\delta \mathcal{F} = \left( \int d\mathcal{A}_s \hat{\mathbf{n}}_1 \cdot \boldsymbol{\Pi} + \mathbf{F}_1^c \right) \cdot \delta \mathbf{R}_1, \quad (\text{S33})$$

where  $\mathcal{A}_s$  and  $\hat{\mathbf{n}}_1$  are the area element and the outward unit normal vector of the colloidal particle, respectively, and the force  $\mathbf{F}_1^c$  is given by

$$\mathbf{F}_1^c \equiv -\frac{\partial}{\partial \mathbf{R}_1} \int d\mathbf{r}' f_{s,1} \epsilon_s |\nabla' \psi_1|^2. \quad (\text{S34})$$

Specifically, consider a particle moving along the  $\hat{\mathbf{z}}$ -direction perpendicular to the planar fluid-fluid interface, in which case  $\delta h \hat{\mathbf{z}} = \delta \mathbf{R}_1$ . Then in the sharp interface limit, we have  $\mathbf{F}_1^c \rightarrow -\partial (\gamma_{1s} A_1 + \gamma_{2s} A_2) / \partial h$ . The change of the free energy reduces to [S25–S27]

$$\delta \mathcal{F} = -\frac{\partial}{\partial h} [-\gamma A_0 + (\gamma_{1s} A_1 + \gamma_{2s} A_2)] \delta h \approx -\gamma \pi d (\cos \theta_s - \cos \theta) \delta h, \quad (\text{S35})$$

with  $A_1 = \pi d h$  and  $A_2 = \pi d (d - h)$  being the particle area in the fluid 1 and fluid 2 domain, respectively, and  $A_0 = \frac{1}{4} \pi [d^2 - (d - 2h)^2]$  being the area of the fluid-fluid interface the particle has displaced. Here  $\gamma = 2\sqrt{2}a\epsilon/3$ ,  $\gamma_{1s}$ , and  $\gamma_{2s}$  are the fluid-fluid, fluid 1-solid, and fluid 2-solid interfacial tensions, respectively,  $\cos \theta_s = (\gamma_{2s} - \gamma_{1s})/\gamma$  being the equilibrium contact angle, and we have used the approximate estimation of the capillary force [S28]  $\delta h \int d\mathcal{A}_s \hat{\mathbf{n}}_1 \cdot \boldsymbol{\Pi} \cdot \hat{\mathbf{z}} = \delta h \int d\mathcal{A}_s K \partial_n \phi \partial_z \phi \approx \gamma \delta A_0$ .

### III. BENCHMARK SIMULATION 1: COMPLICATED (MOVING) SOLID GEOMETRIES

#### A. Governing dynamic equations

In this section, we demonstrate the first advantage of our DRD approach – the capability of simulating viscous flows over solid surfaces that move or have complicated geometries. Specifically, we study the inertial focusing of one (passive, suspending) circular colloidal particle by (single-phase) two-dimensional pressure-driven flows in stationary microchannels without or with surface corrugations, as shown in Fig. S5(a) and Figs. S6(a). In this fluid-solid two-phase flow, the fluid-fluid interface does not exist, so the phase parameter  $\phi$  is not needed to consider, and the only interfacial phase parameters are  $\psi$  for the solid boundaries and  $\psi_1$  for the suspending colloidal particle. Then, from the general dynamic equations presented in Sec. IIB, we obtain the following Navier-Stokes equation:

$$\rho (\partial_t \mathbf{v} + \mathbf{v} \cdot \nabla \mathbf{v}) = -\nabla p + \nabla \cdot [\eta(\mathbf{r}) (\nabla \mathbf{v} + \nabla \mathbf{v}^T)] + \frac{\psi_1 \mathbf{F}_1^{\text{tot}}}{\int d\mathbf{r}' \psi_1}, \quad (\text{S36})$$

supplemented with the incompressibility condition,  $\nabla \cdot \mathbf{v} = 0$ . Here, the total force  $\mathbf{F}_1^{\text{tot}}$  on the particle is applied by the solid boundary and is given from Eq. (S22) by

$$\mathbf{F}_1^{\text{tot}} = -\frac{\partial U_{\text{ps}}}{\partial |\mathcal{D}(\mathbf{R}_1)|} (-\hat{\mathbf{n}}_{s,1}) = -\frac{k_s}{d^2} (|\mathcal{D}(\mathbf{R}_1)| - d/2) (-\hat{\mathbf{n}}_{s,1}), \quad (\text{S37})$$

where  $|\mathcal{D}(\mathbf{R}_1)|$  denotes the minimal distance of the particle at  $\mathbf{r} = \mathbf{R}_1$  away from the solid boundary and it includes the information of complicated solid geometries.  $\hat{\mathbf{n}}_{s,1}$  is the outward unit vector of the solid surface closest to the particle (pointing toward the solid domain). Fluid slip is neglected at all solid boundaries and hence we take the spatially-varying viscosity  $\eta(\mathbf{r})$  in the form of Eq. (S10a) as

$$\eta(\psi, \psi_1) = \eta_f + (\eta_s - \eta_f) (\psi + \psi_1), \quad (\text{S38})$$

where the interfacial profile functions  $\psi$  (of the solid boundary) and  $\psi_1$  (of the particle) both take the form of Eq. (S9):

$$\psi(\mathbf{r}) = \frac{1}{2} \left[ 1 + \tanh \left( \frac{\mathcal{D}(\mathbf{r})}{\sqrt{2}\epsilon_s} \right) \right], \quad \psi_1(\mathbf{r}, t) = \frac{1}{2} \left[ 1 + \tanh \left( \frac{d/2 - |\mathbf{r} - \mathbf{R}_1(t)|}{\sqrt{2}\epsilon_s} \right) \right], \quad (\text{S39})$$

with the particle center  $\mathbf{R}_1(t)$  evolving as Eq. (S14) by

$$\dot{\mathbf{R}}_1 = \mathbf{V}_1(t) = \frac{\int d\mathbf{r}' \psi_1 \mathbf{v}(\mathbf{r}', t)}{\int d\mathbf{r}' \psi_1}. \quad (\text{S40})$$

In addition, we employ the parabolic profile of the inlet velocity at  $x = 0$  to induce the pressure-driven flows inside the microchannel:

$$\mathbf{v}|_{x=0} = V_0 (z(H - z)/(H/2)^2). \quad (\text{S41})$$

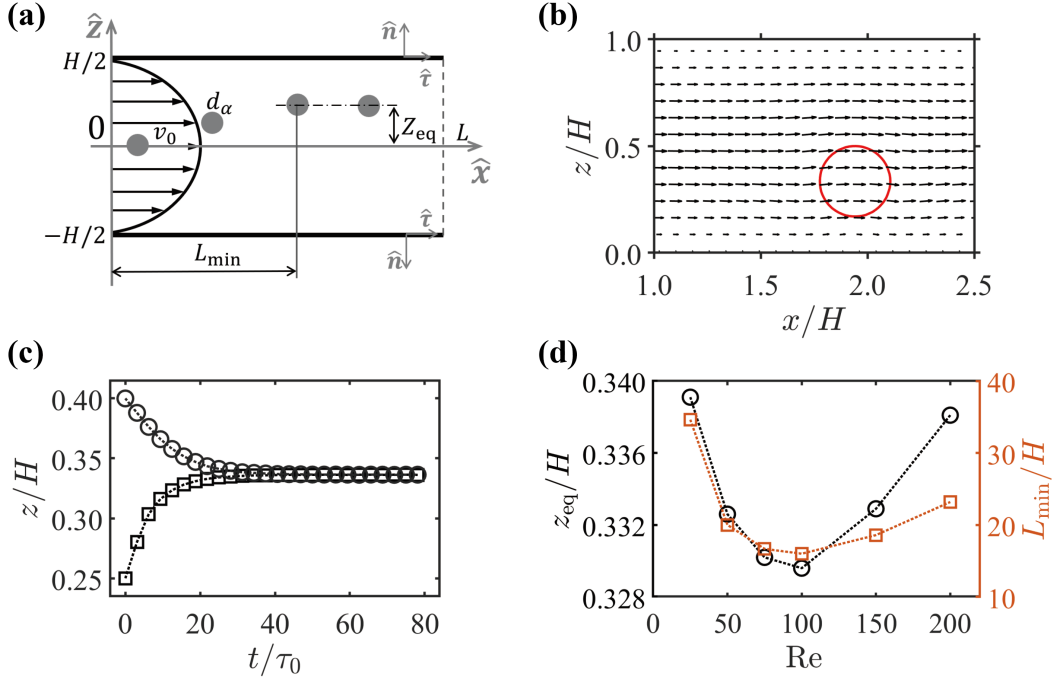

FIG. S5. Inertial focusing of one (passive, suspending) circular colloidal particle by (single-phase) 2D pressure-driven flows in a microchannel with planar surfaces. (a) Schematic illustration of the simulation setup. (b) Flow fields near the particle that has already been focused at equilibrium position  $z_{eq}$ . (c) Equilibration (after  $30\tau_0$ ) of two particles starting from two different initial positions ( $z$ -coordinates) at the inlet boundary  $x = 0$ . (d) Dependence of equilibrium position  $z_{eq}$  and equilibration distance  $L_{min}$  on Reynolds number  $Re = \rho V_0 H / \eta_f$ . Here  $d/H = 1/3$ ,  $L/H = 6.0$ ,  $H = 1.0$ , and periodic boundary conditions have been used in the  $x$ -direction.

### B. Particle focusing in 2D microchannels

Before carrying out simulations, we first non-dimensionalize the above dynamic equations by taking the length unit to be the channel width  $H$ , velocity unit to be the maximal inlet velocity  $V_0$ , time by  $\tau_0 = H/V_0$ , pressure or stress by  $\eta_f V_0/H$ , and force by  $\eta_f V_0$ . Five dimensionless parameters appear as follows.

(1) Reynolds number,  $Re \equiv \rho V_0 H / \eta_f$ , or, the particle Reynolds number:  $Re_p \equiv \rho V_0 d / \eta_f$ . Alternatively, we can define another particle Reynolds number:  $Re_{ps} = \rho V_0 d^2 / \eta_f H$ . It is the characteristic particle Reynolds number in shear flows [S29, S30], which is the ratio of inertial forces  $\rho(2V_0 d/H)^2(d/2)$  to hydrodynamic shear force  $2\eta_f V_0 d/H$ .

(2) Dimensionless stiffness parameter for the particle-solid boundary interaction:  $\mathcal{K}_s = k_s / H \eta_f V_0$ . In our simulations, we take  $\mathcal{K}_s$  to be a large constant to avoid overlapping between the particle and the solid boundary.

(3) Solid-to-fluid viscosity ratio:  $r_\eta \equiv \eta_s / \eta_f \gg 1$ .

(4) Relative fluid-solid interface thickness:  $r_{\epsilon_s} \equiv \epsilon_s / d$ .

(5) Confinement strength or particle-diameter to channel width ratio:  $r_d = d/H$  with  $0 \leq r_d \leq 1$ . Particularly,  $r_d \rightarrow 0$  corresponds to the limit of free (no confinement) particle dynamics in shear flows.  $r_d \rightarrow 1$  or  $d \rightarrow H$  corresponds to the strongest (stuck) confinement case.

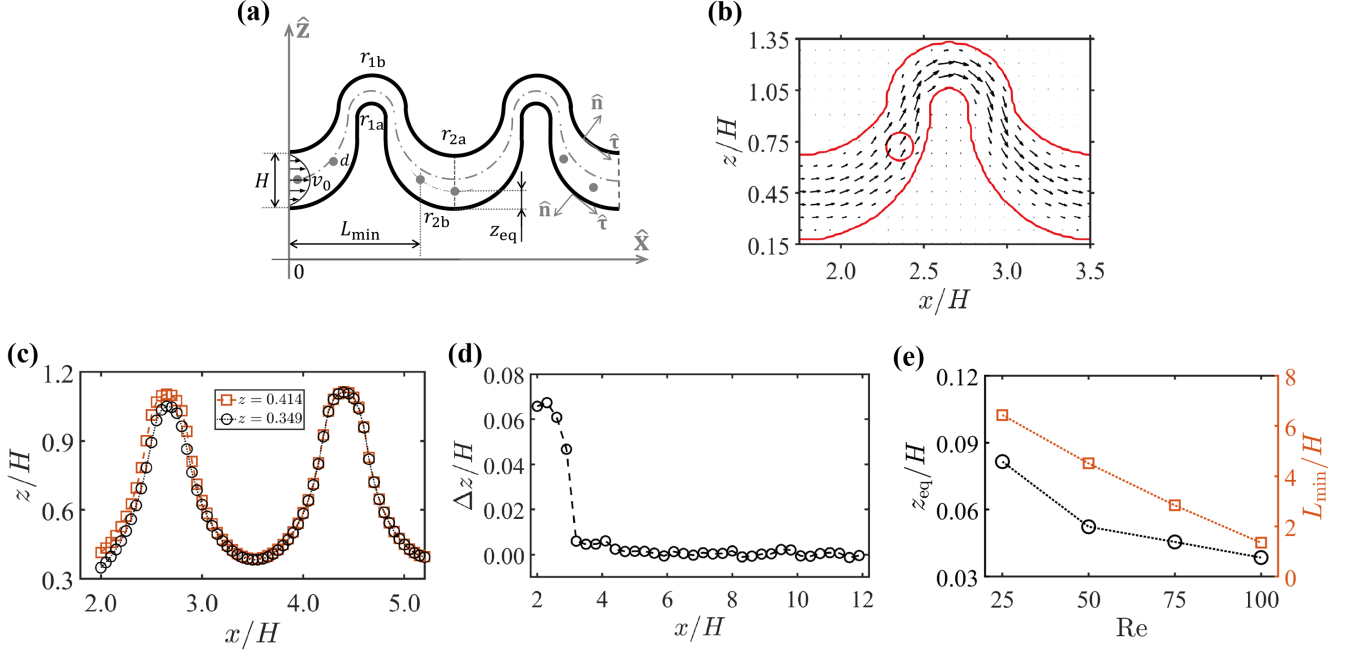

FIG. S6. Inertial focusing of one (passive, suspending) circular colloidal particle by (single-phase) 2D pressure-driven flows in a corrugated (an asymmetrically curved) microchannel. (a) Schematic illustration of the simulation setup. Here the equilibration distance  $L_{\min}$  refers to the minimum length in the  $x$ -direction when the particle is focused, and the equilibrium position  $z_{eq}$  denotes (after the particle being focused) the distance of the particle away from the channel bottom surface as it passes through the middle of the channel at  $x = L_x/2$  with  $L_x$  being the total length of the channel in the  $x$ -direction. (b) Flow fields near the particle that has already been focused at equilibrium position  $z_{eq}$ . (c) Equilibration (after  $30\tau_0$ ) of two particles starting from two different initial positions ( $z$ -coordinate) at the inlet boundary  $x = 0$ . The trajectories of the two particles gradually converge or coincide. (d) A further illustration of equilibration of the two particles starting from two different initial positions by calculating the difference  $\Delta z$  in the  $z$ -coordinates of two particles when they are passing the same  $x$  position. (e) Dependence of the equilibrium position  $z_{eq}$  and the equilibration distance  $L_{\min}$  on Reynolds number  $Re = \rho V_0 H / \eta_f$ . Here  $d/H = 1/3$ ,  $L/H = 7.0$ ,  $H = 0.5$ , and periodic boundary conditions have been used in the  $x$ -direction.

In this study, only two-dimensional simulations are carried out in the  $x$ - $z$  plane as shown in Fig. S5 and Fig. S6. The length and characteristic width of the microchannel are denoted by  $L$  and  $H$ , respectively.

To demonstrate the power of the DRD approach in overcoming the challenges of simulating mFSI involving moving complicated solid geometries, we validate it by simulating the inertial focusing of rigid circular particles in 2D microchannels of planar and corrugated surfaces as shown in Fig. S5 and Fig. S6, respectively. Firstly, for particles in planar microchannels, the particles are focused after traveling a distance of  $L_{\min}$  on a unique equilibrium position  $z_{eq}$  that is independent of the initial positions of the particle but shows a non-monotonic dependence on the Reynolds number  $Re = \rho V_0 H / \eta_f$ . The results agree well with those obtained from other DNS methods in previous works [S31, S32].

Secondly, for inertial particle focusing in 2D corrugated (asymmetrically curved) microchannels, the particles are also found to focus after traveling a distance of  $L_{\min}$  on some equilibrium position that is independent of the initial positions of the particle but shows a monotonic dependence on the Reynolds number  $Re = \rho V_0 H / \eta_f$ . In comparison to that in planar microchannels,  $L_{\min}$  is ten times smaller in corrugated microchannels, that is, channel corrugation increases the efficiency of particle focusing significantly as reported in previous experimental work [S33].

#### IV. BENCHMARK SIMULATION 2: DEFORMABLE (ACTIVE) OBJECTS

##### A. Governing dynamic equations

In this section, we demonstrate the second advantage of our DRD approach – the capability of simulating hydrodynamic interactions between viscous fluids and (active) deformable objects. We combine the DRD approach with particle-based models of (active) deformable objects that have already been widely used in particle-based molecular

simulations in soft matter and biological physics [S14, S34]. Specifically, we consider the following fluid-solid two-phase flow: dynamics of active or passive, deformable or rigid objects in two-dimensional (single-phase) viscous shear flows, as shown in Fig. S8. In this fluid-solid two-phase flow, the fluid-fluid interface also does not exist, so the phase parameter  $\phi$  is not needed, and the only interfacial phase parameters are  $\psi$  for solid boundaries and  $\psi_\alpha$  (with  $\alpha = 1, \dots, N$ ) for the rigid particles that compose the deformable object. Then, from the general dynamic equations presented in Sec. IIB, we obtain the following Navier-Stokes equation:

$$\rho(\partial_t \mathbf{v} + \mathbf{v} \cdot \nabla \mathbf{v}) = -\nabla p + \nabla \cdot [\eta(\mathbf{r})(\nabla \mathbf{v} + \nabla \mathbf{v}^T)] + \sum_{\alpha=1}^N \frac{\psi_\alpha \mathbf{F}_\alpha^{\text{tot}}}{\int d\mathbf{r}' \psi_\alpha}, \quad (\text{S42})$$

supplemented with the incompressibility condition,  $\nabla \cdot \mathbf{v} = 0$ . Here, the total force  $\mathbf{F}_\alpha^{\text{tot}}$  applied on the  $\alpha$ -th particle are given by Eq. (S22) as

$$\mathbf{F}_\alpha^{\text{tot}} \equiv \mathbf{F}_\alpha^{\text{act}} - \sum_{\beta \neq \alpha} \frac{\partial U_{\text{pp}}}{\partial \mathbf{R}_{\beta\alpha}} \hat{\mathbf{R}}_{\beta\alpha} - \frac{\partial U_{\text{ps}}}{\partial |\mathcal{D}(\mathbf{R}_\alpha)|} (-\hat{\mathbf{n}}_{\text{s},\alpha}). \quad (\text{S43})$$

In the simulations of active deformable objects, we also take the simple harmonic form of the particle-solid boundary interaction potential  $U_{\text{ps}}$  in Eq. (S21c). However, the specific form of  $U_{\text{pp}}$  depends on the specific particle-based model of the specific active deformable objects that will be discussed in the following subsections.

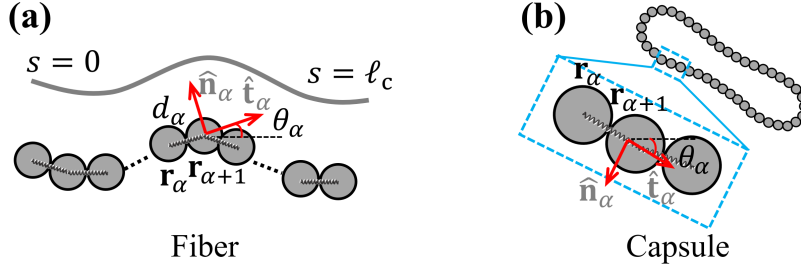

FIG. S7. (Color online) Schematic illustration of deformable objects composed of rigid particles. (a) A flexible fiber and (b) an elastic capsule composed of connected rigid particles using bead-spring model.

## B. Particle-based models for deformable (active) objects

### 1. Flexible fibers: Bead-spring model

A passive flexible fiber can be simulated using the bead-spring model [S14, S35]. As shown schematically in Fig. S7(a), the fiber consists of  $N$  identical rigid circular beads (of diameter  $d$ ) that are connected by  $(N-1)$  identical springs (of equilibrium length  $\ell_0$ ). Flexible fibers show elastic resistance to both compression and bending. In this case, the interactions between fiber bead particles are represented by the following form of energy (per length in 2D):

$$U_{\text{pp}}(\mathbf{R}_\alpha) = \sum_{\alpha=1}^{N-1} \frac{k_s}{2\ell_0^2} (R_{\alpha,\alpha+1} - \ell_0)^2 - \sum_{\alpha=1}^{N-1} k_b (\hat{\mathbf{t}}_{\alpha+1} \cdot \hat{\mathbf{t}}_\alpha)^2. \quad (\text{S44})$$

Here  $R_{\alpha,\alpha+1} = |\mathbf{R}_{\alpha,\alpha+1}|$  is the distance between the center-of-mass of the two neighboring beads with  $\mathbf{R}_{\alpha,\alpha+1} = \mathbf{R}_{\alpha+1} - \mathbf{R}_\alpha$  and  $\mathbf{R}_\alpha$  being the center-of-mass position of each bead.  $\hat{\mathbf{t}}_\alpha = \mathbf{R}_{\alpha,\alpha+1}/R_{\alpha,\alpha+1}$  is tangential unit vector of the fiber.  $k_s$  is the spring constant, and for inextensible fibers, a very large  $k_s$  should be used such that the spring length is close to its equilibrium length  $\ell_0$ , and hence the contour length of the fiber is also almost constant to be  $\ell_c = N\ell_0$ .  $k_b$  is the bending constant that characterizes the bending stiffness of the fiber.

Substituting the energy  $U_{\text{pp}}$  in Eq. (S44) into Eq. (S43) and using  $U_{\text{ps}}$  in Eq. (S21c), we obtain the total force applied on each particle bead of the flexible fiber to be

$$\mathbf{F}_\alpha^{\text{tot}} = \mathbf{F}_\alpha^{\text{s}} + \mathbf{F}_\alpha^{\text{b}} - \frac{k_s}{d^2} (|\mathcal{D}(\mathbf{R}_\alpha)| - d/2) (-\hat{\mathbf{n}}_{\text{s},\alpha}), \quad (\text{S45})$$



in which the lateral spring force  $\mathbf{F}_\alpha^s$  is given by

$$\mathbf{F}_\alpha^s = -\frac{k_s}{\ell_0^2} [(R_{\alpha-1,\alpha} - \ell_0) \hat{\mathbf{t}}_{\alpha-1} - (R_{\alpha,\alpha+1} - \ell_0) \hat{\mathbf{t}}_\alpha], \quad \text{for } 2 \leq \alpha \leq N-1, \quad (\text{S46a})$$

$$\mathbf{F}_1^s = \frac{k_s}{\ell_0^2} (R_{1,2} - \ell_0) \hat{\mathbf{t}}_1, \quad \mathbf{F}_N^s = -\frac{k_s}{\ell_0^2} (R_{N-1,N} - \ell_0) \hat{\mathbf{t}}_{N-1}, \quad (\text{S46b})$$

and the bending force  $\mathbf{F}_\alpha^b$  is given by

$$\mathbf{F}_\alpha^b = k_b \left[ (\hat{\mathbf{t}}_\alpha + \hat{\mathbf{t}}_{\alpha-2}) \cdot \frac{(\mathbf{I} - \hat{\mathbf{t}}_{\alpha-1} \hat{\mathbf{t}}_{\alpha-1})}{R_{\alpha-1,\alpha}} - (\hat{\mathbf{t}}_{\alpha+1} + \hat{\mathbf{t}}_{\alpha-1}) \cdot \frac{(\mathbf{I} - \hat{\mathbf{t}}_\alpha \hat{\mathbf{t}}_\alpha)}{R_{\alpha,\alpha+1}} \right], \quad \text{for } 3 \leq \alpha \leq N-2, \quad (\text{S47a})$$

$$\mathbf{F}_1^b = -k_b \hat{\mathbf{t}}_2 \cdot \frac{(\mathbf{I} - \hat{\mathbf{t}}_1 \hat{\mathbf{t}}_1)}{R_{1,2}}, \quad \mathbf{F}_N^b = k_b \hat{\mathbf{t}}_{N-2} \cdot \frac{(\mathbf{I} - \hat{\mathbf{t}}_{N-1} \hat{\mathbf{t}}_{N-1})}{R_{N-1,N}}. \quad (\text{S47b})$$

$$\mathbf{F}_2^b = k_b \left[ \hat{\mathbf{t}}_2 \cdot \frac{(\mathbf{I} - \hat{\mathbf{t}}_1 \hat{\mathbf{t}}_1)}{R_{1,2}} - (\hat{\mathbf{t}}_3 + \hat{\mathbf{t}}_1) \cdot \frac{(\mathbf{I} - \hat{\mathbf{t}}_2 \hat{\mathbf{t}}_2)}{R_{2,3}} \right], \quad (\text{S47c})$$

$$\mathbf{F}_{N-1}^b = k_b \left[ (\hat{\mathbf{t}}_{N-1} + \hat{\mathbf{t}}_{N-3}) \cdot \frac{(\mathbf{I} - \hat{\mathbf{t}}_{N-2} \hat{\mathbf{t}}_{N-2})}{R_{N-2,N-1}} - \hat{\mathbf{t}}_{N-2} \cdot \frac{(\mathbf{I} - \hat{\mathbf{t}}_{N-1} \hat{\mathbf{t}}_{N-1})}{R_{N-1,N}} \right], \quad (\text{S47d})$$

with  $\mathbf{I}$  being the 2D unit tensor.

## 2. Active (self-propelled) microswimmers: Dumbbell model

Next, to model self-propelling microswimmers, we employ the dumbbell force-dipole model proposed by Furukawa *et al.* [S36], where a swimming microorganism comprises a dumbbell with a pair of prescribed dipolar force (see Fig. S8(a)). Each dumbbell microswimmer consists of one spherical body particle with diameter  $d_B$  and one “phantom” particle with diameter  $d_P$ . The phantom particle can be thought of as a far-field modeling the effect of a thin flagellar bundle, whereby a force is exerted on the fluid at the position with a distance  $d_0$  away from the microswimmer’s body. The propulsion force  $-\mathbf{F}_\alpha^{\text{act}} = F_0 \hat{\mathbf{u}}_\alpha$  is exerted on the fluid via & at the phantom particle; an equal and opposite force  $\mathbf{F}_\alpha^{\text{act}} = F_0 \hat{\mathbf{u}}_\alpha$  is exerted on the body particle, which ensures the dipolar character of the swimming mechanism. Here the active propulsion force is assumed to be applied along the direction of unit vector  $\hat{\mathbf{u}}_\alpha = (\mathbf{R}_\alpha^B - \mathbf{R}_\alpha^P) / |\mathbf{R}_\alpha^B - \mathbf{R}_\alpha^P|$ , where  $\mathbf{R}_\alpha^m$  denotes the position of the particles and the distances of separation between them determine the shape of the microswimmer, where the subscripts  $m = B$  and  $P$  denote the body particles and the phantom particle of the dumbbell, respectively. Particularly, in 2D, we can represent  $\hat{\mathbf{u}}_\alpha$  by  $\hat{\mathbf{u}}_\alpha = (\cos \theta_\alpha, \sin \theta_\alpha)$  with  $\theta_\alpha$  denoting the angle of  $\hat{\mathbf{u}}_\alpha$  relative to the  $+\hat{\mathbf{x}}$  direction.

Since each microswimmer is composed of two particles, it is more convenient to use the following alternative form of dynamic equation (instead of Eq. (S42)):

$$\rho (\partial_t \mathbf{v} + \mathbf{v} \cdot \nabla \mathbf{v}) = -\nabla p + \nabla \cdot [\eta(\mathbf{r}) (\nabla \mathbf{v} + \nabla \mathbf{v}^T)] + \sum_{\alpha=1}^N \sum_{m=B,P} \frac{\psi_\alpha^m \mathbf{F}_\alpha^m}{\int d\mathbf{r} \psi_\alpha^m}, \quad (\text{S48})$$

and the incompressibility condition  $\nabla \cdot \mathbf{v} = 0$ . Here the forces  $\mathbf{F}_\alpha^m$  (with  $m = B, P$  for body and phantom particles, respectively) applied on the center-of-mass of each microswimmer particle are given (from Eq. (S22)) by

$$\mathbf{F}_\alpha^B = \mathbf{F}_\alpha^{\text{act}} - \sum_{\beta \neq \alpha} \frac{\partial U_{\text{pp}}}{\partial R_{\beta\alpha}^B} \hat{\mathbf{R}}_{\beta\alpha}^B - \frac{\partial U_{\text{ps}}}{\partial |\mathcal{D}(\mathbf{R}_\alpha^B)|} (-\hat{\mathbf{n}}_{s,\alpha}^B), \quad \mathbf{F}_\alpha^P = -\mathbf{F}_\alpha^{\text{act}}, \quad (\text{S49})$$

with  $\hat{\mathbf{n}}_{s,\alpha}^B$  being the outward unit vector of the solid surface closest to the body of the  $\alpha$ -th microswimmer (pointing toward the solid domain),  $\mathbf{R}_{\beta\alpha}^B \equiv \mathbf{R}_\alpha^B - \mathbf{R}_\beta^B$ ,  $R_{\beta\alpha}^B \equiv |\mathbf{R}_{\beta\alpha}^B|$ , and  $\hat{\mathbf{R}}_{\beta\alpha}^B \equiv \mathbf{R}_{\beta\alpha}^B / R_{\beta\alpha}^B$ . The particle-solid boundary interaction potential  $U_{\text{ps}}$  is taken to be the simple harmonic form as given in Eq. (S21c).

For the active force  $\mathbf{F}_\alpha^{\text{act}} = F_0 \hat{\mathbf{u}}_\alpha$  that is stochastic and drives the self-propulsion of the microswimmer, we assume it follows run-and-tumble (RTP) dynamics where the magnitude  $F_0$  is constant but the direction of  $\mathbf{F}_\alpha^{\text{act}}$  or  $\hat{\mathbf{u}}_\alpha$  randomly undergoes complete reorientations (“tumbles”) at a certain rate [S37]. The time interval  $\Delta t$  between two subsequent tumbling is chosen using an exponential distribution  $P(\Delta t) = \tau_p^{-1} e^{-\Delta t/\tau_p}$  with  $\tau_p$  being the persistent time. When this time is reached, the microswimmer tumbles, a new orientation  $\hat{\mathbf{u}}_\alpha$  is chosen uniformly in all 3D directions, or in 2D the orientation angle  $\theta_\alpha$  is chosen uniformly in  $[0, 2\pi]$ , and then a new time interval  $\Delta t$  is generated again from the same exponential distribution. In addition, we assume there are no interactions between phantom particles of different microswimmers, which therefore can overlap. However, an overlap between the body and phantom particles of different microswimmers leads to an unphysical effect [S36]. Therefore, we assume that if the phantom particle of the  $\alpha$ -th microswimmer overlaps with the “body” of another  $\beta$ -th microswimmer, that is, when  $|\mathbf{R}_\alpha^{\text{P}} - \mathbf{R}_\beta^{\text{B}}| < (d_{\text{B}} + d_{\text{P}})/2$ , the active force  $\mathbf{F}_\alpha^{\text{act}}$  applied on the  $\alpha$ -th microswimmer will be switched off by setting  $F_0 = 0$  until its phantom particle once again lies in a purely fluid region [S36]. Similar switch rules also apply to the overlap of the phantom particle with the solid boundary. On the other hand, the body particles of different microswimmers should not overlap and exclude each other, and we take the (excluded volume) interactions  $U_{\text{pp}}$  between the body particles of different microswimmers to be a simple harmonic form as given in Eq. (S21b):

$$U_{\text{pp}}(\{R_{\beta\alpha}^{\text{B}}\}) = \sum_{\beta \neq \alpha} \begin{cases} \frac{k_{\text{s}}}{2d^2} (R_{\beta\alpha}^{\text{B}} - d)^2, & R_{\beta\alpha}^{\text{B}} \leq d, \\ 0, & R_{\beta\alpha}^{\text{B}} > d. \end{cases} \quad (\text{S50})$$

with  $k_{\text{s}}$  being the interaction stiffness. Fluid slip is neglected at all particle surfaces and at solid boundaries and hence we take the spatially-varying viscosity  $\eta(\mathbf{r})$  in the form of Eq. (S10a) as

$$\eta(\psi, \psi_1) = \eta_{\text{f}} + (\eta_{\text{s}} - \eta_{\text{f}}) \left( \psi + \sum_{\alpha=1}^N \psi_B^\alpha \right), \quad (\text{S51})$$

where the interfacial profile function  $\psi$  of the solid boundary takes the form of Eq. (S9) and the interfacial profile function  $\psi_\alpha^m$  of the particle takes the form of Eq. (S13) as

$$\psi_\alpha^m(\mathbf{r}, t) = \frac{1}{2} \left[ 1 + \tanh \left( \frac{d_m/2 - |\mathbf{r} - \mathbf{R}_\alpha^m(t)|}{\sqrt{2}\epsilon_s} \right) \right], \quad (\text{S52})$$

with  $\mathbf{R}_\alpha^m(t)$  being the center position of the body particle ( $m = \text{B}$ ) and the phantom particle ( $m = \text{P}$ ) of  $\alpha$ -th microswimmer. The positions  $\mathbf{R}_\alpha^m$  of the microswimmer’s body and phantom particles are updated using the body-particle velocity  $\mathbf{V}_\alpha^{\text{B}}(t)$  and the orientation  $\hat{\mathbf{u}}_\alpha(t)$  of the microswimmer

$$\dot{\mathbf{R}}_\alpha^{\text{B}} = \mathbf{V}_\alpha^{\text{B}}(t) \equiv \frac{\int d\mathbf{r}' \psi_\alpha^{\text{B}} \mathbf{v}(\mathbf{r}', t)}{\int d\mathbf{r}' \psi_\alpha^{\text{B}}}, \quad \mathbf{R}_\alpha^{\text{P}}(t) = \mathbf{R}_\alpha^{\text{B}}(t) - d_0 \hat{\mathbf{u}}_\alpha(t), \quad (\text{S53})$$

respectively.

### C. Far-field dipolar flow field surrounding dumbbell microswimmers

As done in Sec. III B, we non-dimensionalize the above dynamic equations. In addition to the five dimensionless parameters,  $\text{Re} \equiv \rho V_0 H / \eta_{\text{f}}$  or  $\text{Re}_{\text{p}} \equiv \rho V_0 d / \eta_{\text{f}}$  or  $\text{Re}_{\text{ps}} = \rho V_0 d^2 / \eta_{\text{f}} H$ ;  $\mathcal{K}_{\text{s}} = k_{\text{s}} / H \eta_{\text{f}} V_0$ ;  $r_\eta \equiv \eta_{\text{s}} / \eta_{\text{f}} \gg 1$ ;  $r_{\epsilon_{\text{s}}} \equiv \epsilon_{\text{s}} / d$ ;  $r_{\text{d}} = d / H$ , as given in Sec. III B, one more dimensionless parameter arises:  $\mathcal{K}_{\text{b}} = k_{\text{b}} / H \eta_{\text{f}} V_0$ , the stiffness parameter for the fiber bending resistance.

To apply the DRD approach to simulate mFSI in active matter hydrodynamics, we first validated the DRD approach by simulating the flow field generated by a dumbbell microswimmer (see Fig. S8(a)), which is known as a “pusher” and the far-field flow field surrounding the pusher (centered at the origin) is approximated by that of a point force dipole [S36]

$$\mathbf{v}(\mathbf{r}) = \frac{d_0 F_0}{4\pi\eta_{\text{f}}} \frac{2(\hat{\mathbf{r}} \cdot \hat{\mathbf{u}}_\alpha)^2 - 1}{|\mathbf{r}|} \hat{\mathbf{r}}, \quad (\text{S54})$$

where  $\hat{\mathbf{r}} = \mathbf{r}/|\mathbf{r}|$ , and  $\mathbf{r}$  is the distance vector relative to the center of the dipole. In Fig. S8(b), the flow field at a distance of several swimmer body-lengths is shown to match the dipolar flow field given in Eq. (S54) very well.

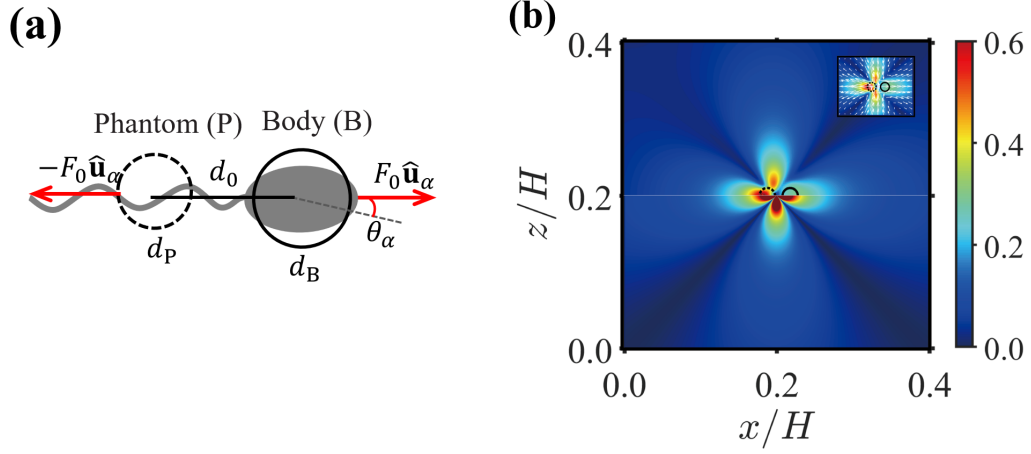

FIG. S8. (Color online) (a) A dumbbell model microswimmer composed of a body particle with diameter  $d_B$  and a “phantom” particle with diameter  $d_P$ . The center-to-center distance between the body particle and the phantom particle is fixed at  $d_0$ . (b) Flow field (top half part) induced by the dumbbell microswimmer (in the reference frame moving with the microswimmer). An analytical far-field flow field induced by an extensible force dipole is also plotted (bottom half part) for comparison. (Inset) The near-field flow in the vicinity of ( $4d_0$  away from) the center of the microswimmer.

## V. BENCHMARK SIMULATION 3: TWO-PHASE FLOWS ON SOLID SURFACES

### A. Governing dynamic equations

In this section, we demonstrate the third advantage of our DRD approach – the capability of simulating multiphase flows on solid surfaces. Specifically, we consider two-phase flows on solid surfaces: moving contact line dynamics of two immiscible two-phase flows on solid surfaces, as shown in Fig. S9. In this triple-phase flow, the fluid-fluid interface and the fluid-solid interface are described by two-phase parameter functions  $\phi$  and  $\psi$ , respectively. In this case, the total free energy is given from Eq. (S15) by

$$\mathcal{F}[\phi(\mathbf{r}), \psi(\mathbf{r})] = \int d\mathbf{r} \left[ f_b(\phi) + \frac{1}{2}K(1-\psi)|\nabla\phi|^2 \right] + \int d\mathbf{r} \epsilon_s f_s(\phi) |\nabla\psi|^2, \quad (\text{S55})$$

where  $f_b(\phi) = \frac{1}{4}a(\phi^2 - 1)^2$  is the double-well potential and  $f_s(\phi) = -\frac{1}{4}\gamma \cos \theta_s(\phi^3 - 3\phi)$  is the surface energy densities at the fluid-particle interface with  $\theta_s$  being the static contact angle at the particle surface. The dissipation function is given by Eq. (S24) and then from the minimization of the Rayleighian  $\mathcal{R}[\mathbf{v}, \mathbf{J}] = \dot{\mathcal{F}}_T + \Phi - \int d\mathbf{r} p \nabla \cdot \mathbf{v}$  in Eq. (S25) with respect to  $\mathbf{v}$  and  $\mathbf{J}$  gives dynamic equations similar to Eqs. (S26):

$$\rho(\partial_t \mathbf{v} + \mathbf{v} \cdot \nabla \mathbf{v}) = -\nabla p + \nabla \cdot [\eta(\nabla \mathbf{v} + \nabla \mathbf{v}^T)] + \hat{\mu}_T \nabla \phi, \quad (\text{S56a})$$

$$\partial_t \phi + \mathbf{v} \cdot \nabla \phi = \nabla \cdot (M \nabla \hat{\mu}_T), \quad (\text{S56b})$$

and the incompressibility condition  $\nabla \cdot \mathbf{v} = 0$ , which are supplemented with proper initial and boundary conditions at the boundary of the computational domain. Here the total chemical potential,  $\hat{\mu}_T$  defined in Eq. (S18) reduces to

$$\hat{\mu}_T = \hat{\mu} + \epsilon_s \mu_s |\nabla \psi|^2, \quad (\text{S57})$$

with  $\hat{\mu} = \mu - \nabla \cdot [K(1-\psi)\nabla\phi]$ ,  $\mu = a\phi(\phi^2 - 1)$ , and  $\mu_s = -\frac{3}{4}\gamma \cos \theta_s(\phi^2 - 1)$  being the generalized chemical potential for two-phase fluids, the chemical potential for homogeneous fluids, and the surface chemical potentials at solid boundary surfaces, respectively. Moreover, since fluid slip and relaxation dissipation across the fluid-solid interface are both critical in multiphase dynamics, particularly, in the contact line motion [S4], Therefore, we choose the non-monotonic smooth profiles of viscosity  $\eta(\mathbf{r})$  and mobility  $M(\mathbf{r})$  given in Eq. (S11). The interfacial profile function  $\psi$  of the solid boundary takes the general form of Eq. (S9).

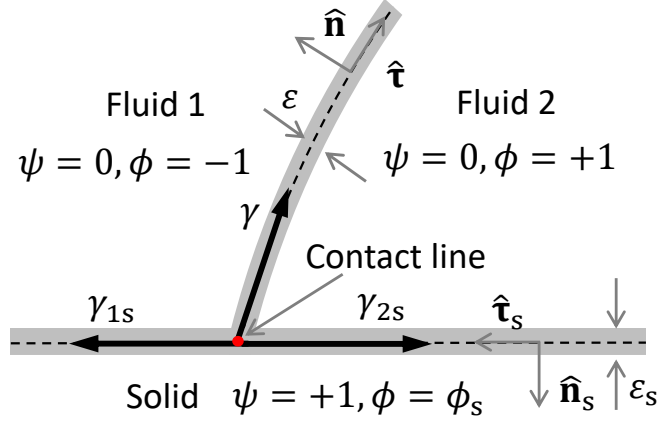

FIG. S9. Schematic illustration for the moving contact line in immiscible two-phase flows on a planar solid surface. The immiscible two-phase fluid domain is distinguished by different values of  $\phi$  while sharing the same value  $\psi$ . The solid domain is represented by  $\psi = 1$  and  $\phi = \phi_s$ .

### B. Sharp-interface limit and generalized Navier boundary conditions (GNBC)

Now we consider the sharp-interface limit of the general dynamics equations in Sec. V A that are derived based on the diffuse fluid-solid interface, from which we show that generalized Navier boundary conditions (GNBC) at solid surface derived by Qian *et al.* [S4, S16] can be recovered. For specificity and simplicity, we consider immiscible two-phase flows over a rigid solid domain with a planar surface at  $z = 0$  (outward normal direction along  $-\hat{\mathbf{z}}$ -direction) as shown in Fig. S9. In this case, the interfacial profile function  $\psi$  in Eq. (S9) of the solid boundary reduces to a simpler form

$$\psi(z) = \frac{1}{2} \left[ 1 + \tanh \left( \frac{z}{\sqrt{2}\epsilon_s} \right) \right]. \quad (\text{S58})$$

In contrast with traditional mathematical methods of taking sharp-interface limits of dynamic equations, we carry out the sharp-interface limits of the rate of change of the total free energy  $\dot{\mathcal{F}}_T$  in Eq. (S17) and the dissipation function in Eq. (S24).

Noting that the chemical potential  $\hat{\mu} \approx -\partial_z[K(1-\psi)\partial_z\phi]$  across the fluid-solid interface of small thickness  $\epsilon_s$ , we obtain the rate of change of the fluid-solid interface energy  $\dot{\mathcal{F}}_s$  in Eq. (S17)

$$\dot{\mathcal{F}}_s \approx \int d\mathcal{A} \int_{-\epsilon_s}^{+\epsilon_s} dz \left\{ -\partial_z[K(1-\psi)\partial_z\phi] + \epsilon_s \mu_s |\partial_z\psi|^2 \right\} \partial_t \phi \approx \int d\mathcal{A} \left( -K \partial_z \phi + \frac{\partial f_s}{\partial \phi} \right) \partial_t \phi, \quad (\text{S59})$$

where  $d\mathcal{A}$  is the area element of the solid surface, the surface energy density is  $f_s(\phi) = -\frac{1}{4}\gamma \cos \theta_s (\phi^3 - 3\phi)$ , and we have used the identity  $\int_{-\infty}^{+\infty} dz \epsilon_s |\partial_z\psi|^2 = 2\sqrt{2}/3$ . On the other hand, noting that the dominant component of the shear rate tensor is  $\partial_z v_x \sim v_x^{\text{slip}}/\epsilon_s$  and  $\mathbf{J} \approx J_z \hat{\mathbf{z}} \sim -\dot{\phi} \epsilon_s$ , we obtain the dissipation function at the fluid-solid interface from Eq. (S24)

$$\Phi_s[\mathbf{v}, \mathbf{J}] \approx \int d\mathcal{A} \int_{-\epsilon_s}^{+\epsilon_s} dz \left[ \frac{1}{4} \eta_i (\partial_z v_x)^2 + \frac{J_z^2}{2M_i} \right] = \int d\mathcal{A} \left[ \frac{1}{2} \beta (v_x^{\text{slip}})^2 + \frac{\dot{\phi}^2}{2\Gamma} \right], \quad (\text{S60})$$

with  $v_x^{\text{slip}}$  being the slip velocity of the fluids relative to the solid at the solid surface. Here the friction coefficient  $\beta \sim \eta_i/\epsilon_s$  and hence the slip length  $\ell_s = \eta_f/\beta$  relative to fluid-solid interface thickness  $\epsilon_s$  scales as  $\ell_s/\epsilon_s \sim \eta_f/\eta_i$ . On the other hand, the relaxational parameter  $\Gamma \sim M_i/\epsilon_s^3$  and hence the relaxation time  $\tau_s \sim \epsilon_s/K\Gamma$  at the solid surface relative to that  $\tau_f \sim M_f K/\epsilon^4$  in the bulk length scales  $\tau_s/\tau_f \sim M_f/M_i$  (since the thicknesses of fluid-fluid and fluid-solid are of same order  $\epsilon \sim \epsilon_s$ ).

Furthermore, if we combine the change rate of surface energy and surface dissipation at the solid surface in Eqs. (S59) and (S60) with that in the bulk, given by

$$\dot{\mathcal{K}}_b = \int d\mathbf{r} \hat{\mu} \partial_t \phi, \quad \Phi_b[\mathbf{v}, \mathbf{J}] = \int d\mathbf{r} \left[ \frac{1}{4} \eta (\nabla \mathbf{v} + \nabla \mathbf{v}^T)^2 + \frac{\mathbf{J}^2}{2M} \right], \quad (\text{S61})$$

and use  $\dot{\phi} = \partial_t \phi + v_x \partial \phi$  (due to the impermeability condition, imposed by large viscosity in the solid domain in our DRD approach) at the solid surface as well as the incompressibility condition  $\nabla \cdot \mathbf{v} = 0$ , we obtain the Rayleighian,  $\mathcal{R}[\mathbf{v}, \mathbf{J}, v_x^{\text{slip}}, \dot{\phi}] = \dot{\mathcal{F}}_b + \dot{\mathcal{F}}_s + \Phi_b + \Phi_s - \int d\mathbf{r} p \nabla \cdot \mathbf{v}$ , which has been constructed by Qian *et al.* [S4, S16] and the thermodynamically consistent model, including the famous generalized Navier boundary conditions (GNBC), can be recovered completely. Finally, note that if we take the linear monotonic form of  $\eta$  and  $M$  as shown in Eqs. (S10), we will recover the no-slip boundary condition for velocity and equilibrium condition for  $\phi$ , *i.e.*,  $v_x^{\text{slip}} = 0$  and  $-K \partial_z \phi + \partial \gamma_{\text{FS}} / \partial \phi = 0$ .

### C. Equilibrating dynamics of sessile droplets on planar surfaces

As done in Sec. III B, we non-dimensionalize the above dynamic equations by scaling the length by the system width or height  $H$ , velocity by some characteristic velocity  $V_0$ , time by  $\tau_0 \equiv H/V_0$ , pressure and stress by  $\eta_f V_0/H$ , chemical potential by  $a$ , viscosity by  $\eta_f$ , the mobility coefficient by  $M_f$ . Ten major dimensionless parameters appear in the above equation system.

- (1) Reynolds number,  $\text{Re} \equiv \rho V_0 H / \eta_f \ll 1$ .
- (2)  $\mathcal{B} \equiv a H / \eta_f V_0$ , which is inversely proportional to the Capillary number  $\text{Ca} \equiv \eta_f V_0 / \gamma$  with  $\gamma = 2\sqrt{2}a\epsilon/3$ .
- (3)  $m \equiv M_f a / V_0 H$ , which approximates the ratio of the characteristic time  $\tau_0$  to the relaxation time  $H^2/aM_f$ .
- (4,5) Viscosity ratios. Solid-to-fluid viscosity ratio:  $r_\eta \equiv \eta_s / \eta_f \gg 1$ . Interfacial-to-fluid viscosity ratio:  $r_{\eta_i} \equiv \eta_i / \eta_f < 1$ .
- (6,7) Mobility ratios. Solid-to-fluid mobility ratio:  $r_M \equiv M_s / M_f \rightarrow 0$ . Interfacial-to-fluid mobility ratio:  $r_{M_i} \equiv M_i / M_f > 1$ .
- (8,9) Relative interfacial thicknesses. Fluid-fluid interface thickness:  $r_\epsilon \equiv \epsilon / H \ll 1$ . Fluid-solid interface thickness:  $r_{\epsilon_s} \equiv \epsilon_s / H \ll 1$ .
- (10) Static contact angles  $\theta_s \in [0, \pi]$ .

To validate the DRD approach in simulating two-phase flows on solid surfaces, we simulated the equilibrating dynamics of a sessile droplet on planar surfaces with two different static contact angles ( $30^\circ$  and  $150^\circ$ ) as shown in Fig. S10. Starting from the same initial condition at  $t = 0$  of initial contact angle  $90^\circ$ , the droplets are shown to spread or dewet spontaneously and finally equilibrate at the pre-set static contact angles.

## VI. BENCHMARK SIMULATION 4: REACTIVE POROUS-MEDIA FLOWS WITH EVOLVING SOLID SURFACES

### A. Governing dynamic equations

Up to now, we have only considered the three advantages of our DRD approach in simulating mFSI that involve solid domains that are rigid and can be moving or deforming in fluids. In this section, we address another advantage of our DRD approach that it can also be applied to study mFSI where solid structure evolves in time such as that occurs during crystal growth & melting [S38], and precipitation & dissolution in porous-media [S39], *etc.* To be specific, we consider the precipitation & dissolution in an array of solid particles (nucleates) where viscous flows are coupled with solute diffusion in the bulk and precipitation & dissolution at the solid surfaces, as shown in Fig. S11. Such precipitation & dissolution can be regarded as a chemical reaction where the solute molecules in the fluid bulk and those in the solid are two different species transforming through the elementary reaction

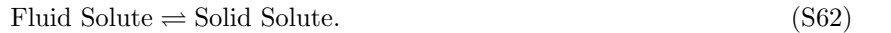

In this case, the fluid is a single-phase solution with diffusing solute concentration  $c$ , while in the solid phase, the solute concentration is always a constant  $c_s$  and the structure or shape of the solid evolves with time.

In this fluid-solid two-phase flow, the fluid-fluid interface also does not exist, so the phase parameter  $\phi$  is not needed, and the only interfacial phase parameter is  $\psi$  for the solid boundary, taking the form of Eq. (S9):

$$\psi(\mathbf{r}, t) = \frac{1}{2} \left[ 1 + \tanh \left( \frac{\mathcal{D}(\mathbf{r}, t)}{\sqrt{2}\epsilon_s} \right) \right].$$

The conservation of solute in the fluid is given by

$$\partial_t c + \mathbf{v} \cdot \nabla c = -\nabla \cdot \mathbf{J} - r_p(1 - c/c_s)|\nabla \psi(\mathbf{r}, t)|, \quad (\text{S63})$$

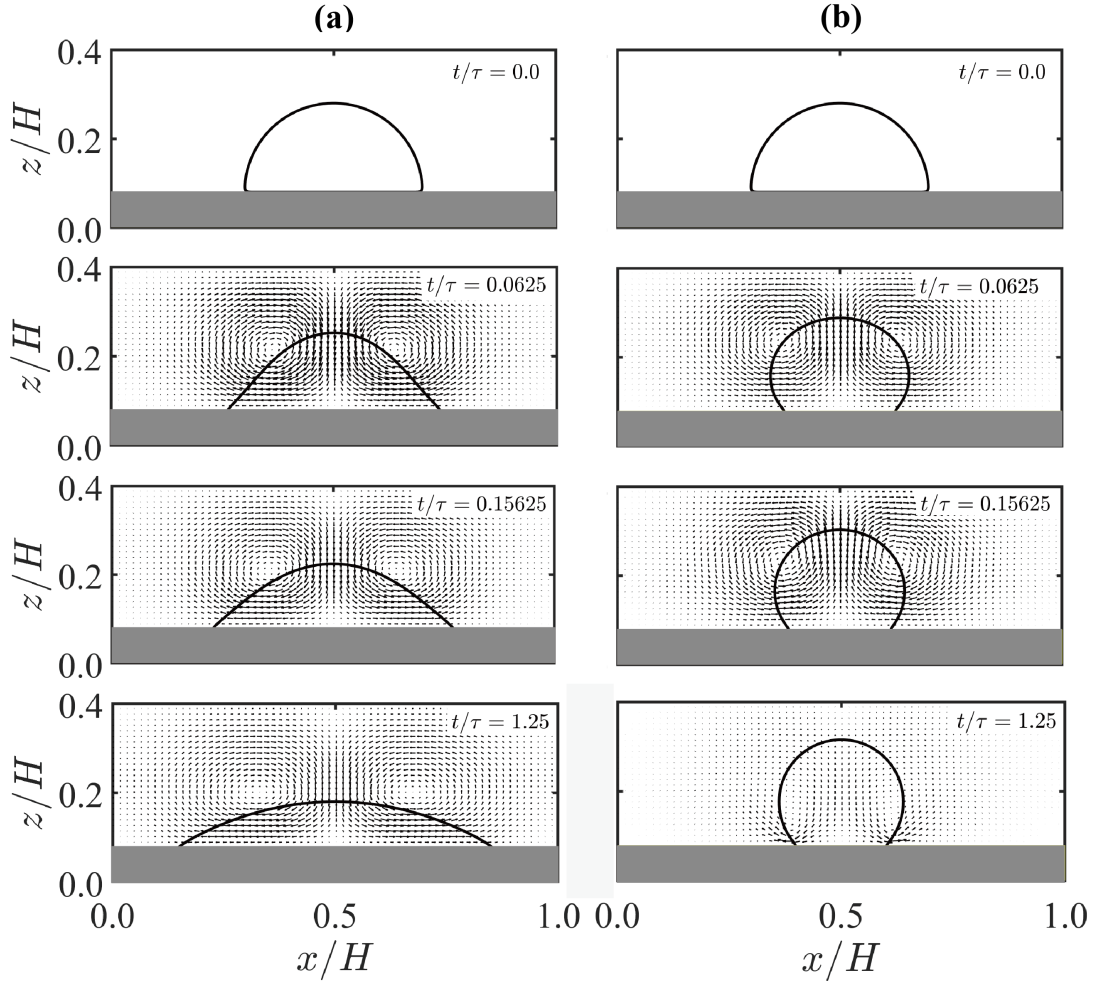

FIG. S10. Equilibrating dynamics of a sessile droplet on planar solid surfaces with two different contact angles: (a)  $30^\circ$  and (b)  $150^\circ$ . The interface profiles (solid curves) of the droplet, the flow fields (arrows), and the solid phase (gray) are all shown in the snapshots of the simulations.

where  $\mathbf{v}$  is the velocity field,  $\mathbf{J}$  is the diffusion flux of fluid/solid solute, and  $r_p$  denotes the net rate of precipitation & dissolution that occurs only at the fluid-solid interface (as indicated by the factor of  $|\nabla\psi(\mathbf{r}, t)|$ ). Moreover, the temporal evolution of solid shape or structure can be represented by the evolution of signed distance function  $\mathcal{D}(\mathbf{r}, t)$ :

$$\partial_t \mathcal{D}(\mathbf{r}, t) + \frac{r_p}{c_s} |\nabla \mathcal{D}(\mathbf{r}, t)| = 0, \quad \text{or,} \quad \partial_t \psi(\mathbf{r}, t) + \frac{r_p}{c_s} |\nabla \psi(\mathbf{r}, t)| = 0. \quad (\text{S64})$$

The free energy of the two-phase system is given by

$$\mathcal{F}[c(\mathbf{r}), \psi(\mathbf{r})] = \int d\mathbf{r} [f(c) + \psi f_s(c_s)], \quad (\text{S65})$$

with  $f(c) = k_B T c \ln c$  and the dissipation function includes contributions from three dissipation mechanisms (viscous dissipation, diffusion, and reaction) as

$$\Phi[\mathbf{v}, \mathbf{J}] = \int d\mathbf{r} \left[ \frac{\eta}{4} (\nabla \mathbf{v} + \nabla \mathbf{v}^T)^2 + \frac{\zeta}{2c} \mathbf{J}^2 + \frac{1}{2\Gamma} r_p^2 |\nabla \psi(\mathbf{r}, t)|^2 \right]. \quad (\text{S66})$$

Imposing the incompressibility condition  $\nabla \cdot \mathbf{v} = 0$ , we obtain the Rayleighian

$$\mathcal{R}[\mathbf{v}, \mathbf{J}] = \dot{\mathcal{F}} + \Phi - \int d\mathbf{r} p \nabla \cdot \mathbf{v}, \quad (\text{S67})$$



with  $p$  being a local Lagrange multiplier and representing pressure. Minimizing  $\mathcal{R}$  with respect to  $\mathbf{v}$ ,  $\mathbf{J}$ , and  $r_p$  gives

$$\rho(\partial_t \mathbf{v} + \mathbf{v} \cdot \nabla \mathbf{v}) = -\nabla p + \nabla \cdot [\eta(\nabla \mathbf{v} + \nabla \mathbf{v}^T)], \quad (\text{S68a})$$

$$\partial_t c + \mathbf{v} \cdot \nabla c = \nabla \cdot (D \nabla c) - r_p(1 - c/c_s)|\nabla \psi(\mathbf{r}, t)|, \quad (\text{S68b})$$

$$\partial_t \psi(\mathbf{r}, t) + \frac{r_p}{c_s} |\nabla \psi(\mathbf{r}, t)| = 0, \quad (\text{S68c})$$

with  $r_p = \Gamma \Delta \mu$ ,  $D = k_B T / \zeta$ , and  $c_s \Delta \mu \equiv f_s - \mu(c - c_s)$  with  $\mu = \partial_c f = k_B T (\ln c + 1)$ . For first-order reaction kinetics [S40], we take

$$r_p = k_r(c^2/c_{\text{eq}}^2 - 1), \quad (\text{S69})$$

with  $k_r$  being a (positive) constant reaction rate and  $c_{\text{eq}} (< c_s)$  being some equilibrium concentration when precipitation or dissolution stops [S40]. Here the smooth profiles of viscosity  $\eta(\mathbf{r})$  and diffusivity  $D(\mathbf{r})$  are taken to be the linear monotonic interpolation form given in Eqs. (S10) as

$$\eta(\psi) = \eta_f + (\eta_s - \eta_f) \psi, \quad D(\psi) = D_f + (D_s - D_f) \psi. \quad (\text{S70})$$

A very large viscosity  $\eta_s (\gg \eta_f)$  and very small diffusivity  $D_s (\ll D_f)$  in the solid domain can reproduce the following boundary conditions in the sharp interface limit:  $\mathbf{v} = \mathbf{0}$  and  $\hat{\mathbf{n}} \cdot D \nabla c = r_p(1 - c/c_s)$ .

Note that we can implement the dynamic equation (S68c) of the evolving solid surfaces by the level-set method and interface breakup or coalescence can be simulated without additional difficulties. Alternatively, we can use the phase-field method through the Cahn-Hilliard dynamics by further extending Eq. (S64) or Eq. (S68c) to be

$$\partial_t \psi(\mathbf{r}, t) - \tau_{\text{sn}}^{-1} \epsilon_s^2 \nabla^2 \mu_\psi + \frac{r_p}{c_s} |\nabla \psi(\mathbf{r}, t)| = 0, \quad (\text{S71})$$

with  $\mu_\psi = (\psi - 3\psi^2 + 2\psi^3) - \epsilon_s^2 \nabla^2 \psi$  being the generalized chemical potential and  $\tau_{\text{sn}}$  is a timescale governing the relaxational dynamics of interface profile that should be chosen to be smaller than  $\epsilon_s c_s / r_p$ .

Before carrying out simulations, we first non-dimensionalize the above dynamic equations by scaling the length by the system width  $H$ , time by characteristic precipitation time  $\tau_{\text{pr}} \equiv H c_s / k_r$ , velocity by  $H / \tau_{\text{pr}}$ , pressure or stress by  $\eta_f / \tau_{\text{pr}}$ , solute concentration by  $c_s$ , viscosity by  $\eta_f$ , and diffusivity by  $D_f$ . Seven major dimensionless parameters appear as follows.

- (1) Reynolds number:  $\text{Re} \equiv \rho H k_r / \eta_f c_s$ .
- (2) Péclet number:  $\text{Pe} \equiv V_0 H / D_f$ .
- (3) Damköhler number:  $\text{Da} \equiv H k_r / D_f c_s$ , or, Karlovitz number:  $\text{Ka} \equiv \text{Da}^{-1}$ .
- (4) Relative mobility parameter:  $\mathcal{M} \equiv \tau_{\text{pr}} / \tau_{\text{sn}} = H c_s / k_r \tau_{\text{sn}}$ .
- (5) Solid-to-fluid viscosity ratio:  $r_\eta \equiv \eta_s / \eta_f \gg 1$ .
- (6) Solid-to-fluid diffusivity ratio:  $r_D \equiv D_s / D_f \rightarrow 0$ .
- (7) Relative fluid-solid interface thickness:  $r_{\epsilon_s} \equiv \epsilon_s / H \ll 1$ .
- (8) Normalized equilibrium (saturation) concentration:  $r_c \equiv c_{\text{eq}} / c_s < 1$ .

## B. Precipitation dynamics in 1D

To validate the DRD approach to simulate mFSI in porous-media flows involving solute precipitations, we simulated the precipitation in a 1D fluid-solid system as shown schematically in Fig. S11(a). In this simple 1D case, we first formulate a sharp interface model as follows for the homogeneous precipitation of an ionic liquid solution onto a solid surface in 1D [S40] with  $0 \leq z \leq H$  and the liquid-solution interface located at  $z = h$ , as shown in Fig. S11. For simplicity, we consider a one-component-solute theory where the ion concentration follows the 1D diffusion equation

$$\partial_t c = D \partial_z^2 c, \quad (\text{S72})$$

supplemented with  $c(H, t) = c_0$  and a Robin-type boundary condition at  $z = h$ :

$$D \partial_z c = r_p(1 - c/c_s), \quad (\text{S73})$$

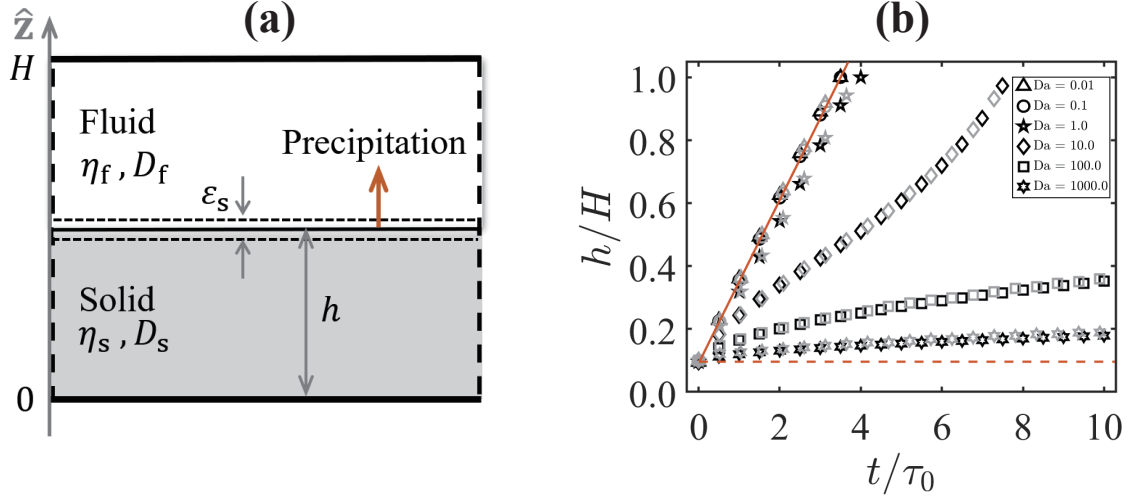

FIG. S11. (a) Schematic illustration for the precipitation & dissolution at the fluid-solid interface in 1D. (b) Comparisons between the numerical solutions obtained from the DRD approach with those from sharp interface models in a large range of Damköhler number:  $Da \equiv k_r H / D_f c_s \in [0.01, 1000]$ .

$$r_p = c_s dh/dt = k_r (c^2/c_{eq}^2 - 1). \quad (S74)$$

In such a 1D sharp-interface precipitation model, there exist two major time scales: (i)  $\tau_D \sim H^2/D_f$ , the characteristic diffusion time of solute in the liquid solution; (ii)  $\tau_{pr} \sim Hc_s/k_r$ , the characteristic precipitating time for the solution. The dimensionless Damköhler number,  $Da \equiv \tau_D/\tau_{pr}$  or the Karlovitz number,  $Ka \equiv Da^{-1}$  are the ratios between the diffusion time and the interfacial precipitation time, which characterize their relative importance in determining a steady-state ion mass distribution and precipitation rate over the length and time scales of interest. Two limiting regimes can be identified according to the magnitude of  $Da$  as follows.

- For  $Da \gg 1$ , or,  $Ka \ll 1$ , or equivalently,  $\tau_{pr} \ll \tau_D$ , the interface-equilibration rate is much larger than the diffusion rate, and the precipitation is said to be *diffusion-limited*. In this case, diffusion is the slowest process so diffusion characteristics dominate and the liquid-solid interface is assumed to be instantaneously in equilibrium. The boundary condition in Eq. (S74) should be replaced by

$$c(h, t) = c_{eq}. \quad (S75)$$

The steady-state solution  $c(z, t \rightarrow \infty)$  and  $h(t)$  (where the timescale  $t$  is much larger than  $\tau_D$  and  $\tau_{pr}$ ) of the above equation system can be found to be

$$c(z) = c_0 - (c_0 - c_{eq}) \frac{H - z}{H - h}, \quad (S76a)$$

$$(H - h(t))^2 = (H - h_0)^2 - 2D \frac{c_0 - c_{eq}}{\rho_s - c_{eq}} t. \quad (S76b)$$

- For  $Da \ll 1$ , or,  $Ka \gg 1$ , or equivalently,  $\tau_{pr} \gg \tau_D$ , diffusion occurs much faster than the interface equilibration, and the precipitation is said to be *reaction-limited*. In this case, diffusion reaches an “equilibrium” well before the interface is at equilibrium. The steady-state solution  $c(z, t \rightarrow \infty)$  and  $h(t)$  (where the timescale  $t$  is much larger than  $\tau_D$  and  $\tau_{pr}$ ) of the above equation system can be expanded in terms of  $Da$  to the first order as

$$c(z) \approx c_0 - Da c_{eq} \left( \frac{c_0^2}{c_{eq}^2} - 1 \right) \left( 1 - \frac{c_0}{\rho_s} \right) \left( 1 - \frac{z}{H} \right), \quad (S77a)$$

$$h(t) \approx h_0 + Da \frac{c_{eq}}{\rho_s} \left( \frac{c_0^2}{c_{eq}^2} - 1 \right) \frac{Dt}{H}. \quad (S77b)$$

Finally, we compared the numerical solutions for  $h(t)$  using the DRD approach with the analytical solutions and numerical solutions of the above sharp interface model. We find very good quantitative agreement between the two solutions in a large range of Damköhler number or Karlovitz number:  $Da \in [0.01, 1000]$  or  $Ka \in [0.001, 100]$  as shown in Fig. S11(b).

## SUPPLEMENTARY REFERENCES

- [S1] L. Onsager, *Phys. Rev.* **37**, 405 (1931).
- [S2] M. Doi, *Prog. Polym. Sci.* **112**, 101339 (2021).
- [S3] H. Wang, T. Qian, and X. Xu, *Soft Matter* **17**, 3634 (2021).
- [S4] T. Qian, X.-P. Wang, and P. Sheng, *J. Fluid Mech.* **564**, 333 (2006).
- [S5] H. Tanaka and T. Araki, *Phys. Rev. Lett.* **85**, 1338 (2000).
- [S6] A. Furukawa, M. Tateno, and H. Tanaka, *Soft Matter* **14**, 3738 (2018).
- [S7] R. Yamamoto, *Phys. Rev. Lett.* **87**, 075502 (2001).
- [S8] I. Mirzaii and M. Passandideh-Fard, *Int. J. Multiph. Flow* **39**, 216 (2012).
- [S9] J. Brannick, C. Liu, T. Qian, and H. Sun, *Numer. Math.-Theory Mes.* **8**, 220 (2015).
- [S10] J. Yang and J. Kim, *Comput. Math. Appl.* **79**, 1857 (2020).
- [S11] M. Carlson, P. J. Mucha, R. B. Van Horn III, and G. Turk, in *Proc. 2002 ACM SIGGRAPH/Eurographics symposium on Computer animation* (2002) pp. 167–174.
- [S12] H. Esmailzadeh and M. Passandideh-Fard, *J. Fluids Eng.* **136**, 111107 (2014).
- [S13] J. Zhang, X. Xu, and T. Qian, *Phys. Rev. E* **91**, 033016 (2015).
- [S14] J. Su, K. Ma, Z. Yan, Q. He, and X. Xu, *Phys. Fluids* **35** (2023).
- [S15] Y. Fujitani, *J. Phys. Soc. Japan* **76**, 064401 (2007).
- [S16] T. Qian, C. Qiu, and P. Sheng, *J. Fluid Mech.* **611**, 333–364 (2008).
- [S17] A. Furukawa, D. Marenduzzo, and M. E. Cates, *Phys. Rev. E* **90**, 022303 (2014).
- [S18] X. Li, J. Lowengrub, A. Rätz, and A. Voigt, *CCommun. Math. Sci.* **7**, 81 (2009).
- [S19] Z. Guo, F. Yu, P. Lin, S. Wise, and J. Lowengrub, *J. Fluid Mech.* **907**, A38 (2021).
- [S20] H. Tanaka and T. Araki, *Chem. Eng. Sci.* **61**, 2108 (2006).
- [S21] H. Wang, B. Zou, J. Su, D. Wang, and X. Xu, *Soft Matter* **18**, 6015 (2022).
- [S22] H. H. Hu, *Int. J. Multiph. Flow* **22**, 335 (1996).
- [S23] G. Tryggvason, R. Scardovelli, and S. Zaleski, *Direct numerical simulations of gas–liquid multiphase flows* (Cambridge university press, 2011).
- [S24] P. Angot, C.-H. Bruneau, and P. Fabrie, *Numerische Mathematik* **81**, 497 (1999).
- [S25] S. Levine, B. D. Bowen, and S. J. Partridge, *Colloids Surf.* **38**, 325 (1989).
- [S26] G. B. Davies, T. Krüger, P. V. Coveney, and J. Harting, *J. Chem. Phys.* **141** (2014).
- [S27] H. Gidituri, A. Würger, K. Stratford, and J. S. Lintuvuori, *Phys. Fluids* **33** (2021).
- [S28] P. C. Millett and Y. U. Wang, *J. Colloid Interface Sci.* **353**, 46 (2011).
- [S29] C. Zettner and M. Yoda, *J. Fluid Mech.* **442**, 241 (2001).
- [S30] H. Huang, X. Yang, M. Krafczyk, and X.-Y. Lu, *J. Fluid Mech.* **692**, 369 (2012).
- [S31] D. V. Esipov, D. V. Chirkov, D. S. Kuranakov, and V. N. Lapin, *Journal of Fluids Engineering* **142**, 111501 (2020).
- [S32] S. R. Bazaz, A. Mashhadian, A. Ehsani, S. C. Saha, T. Krüger, and M. E. Warkiani, *Lab on a Chip* **20**, 1023 (2020).
- [S33] D. Di Carlo, D. Irimia, R. G. Tompkins, and M. Toner, *Proceedings of the National Academy of Sciences* **104**, 18892 (2007).
- [S34] A. Boromand, A. Signoriello, F. Ye, C. S. O’Hern, and M. D. Shattuck, *Phys. Rev. Lett.* **121**, 248003 (2018).
- [S35] S. Yamamoto and T. Matsuoka, *J. Chem. Phys.* **98**, 644 (1993).
- [S36] A. Furukawa, D. Marenduzzo, and M. E. Cates, *Phys. Rev. E* **90**, 022303 (2014).
- [S37] A. P. Solon, Y. Fily, A. Baskaran, M. E. Cates, Y. Kafri, M. Kardar, and J. Tailleur, *Nat. Phys.* **11**, 673 (2015).
- [S38] K. Takae and A. Onuki, *Phys. Rev. E* **83**, 041504 (2011).
- [S39] A. Almajed, M. A. Lateef, A. A. B. Moghal, and K. Lemboye, *Crystals* **11**, 370 (2021).
- [S40] T. Van Noorden and I. Pop, *IMA J. Appl. Math.* **73**, 393 (2008).
